# Supplementary material for: A construction principle for tight and minimal triangulations of manifolds
Source: arXiv:1511.04500 ancillary file (2016-07-11)
Supplement: Supplementary file 1 [file ListOfExamples.pdf]

# Full list of examples from: *A construction principle for tight and minimal triangulations of manifolds*

BENJAMIN A. BURTON<sup>1</sup>, BASUDEB DATTA<sup>2</sup>, NITIN SINGH<sup>3</sup>, JONATHAN SPREER<sup>4</sup>

<sup>1,4</sup>*School of Mathematics and Physics, The University of Queensland, Brisbane QLD 4072, Australia. bab@maths.uq.edu.au, j.spreer@uq.edu.au.*

<sup>2</sup>*Department of Mathematics, Indian Institute of Science, Bangalore 560 012, India. dattab@math.iisc.ernet.in.*

<sup>3</sup>*IBM India Research Lab, Bangalore 560 045, India. nitisin1@in.ibm.com.*

June 20, 2016

---

## Abstract

This document contains the full list of the sporadic examples of tight and minimal triangulations of handlebodies presented in [1]. The complexes will also be available from within the GAP-package `simpcomp` [2, 3] via functions `SCNrTightHandleBodies(d,k)` and `SCTightHandleBody(d,k,idx)` as of the next update. Please refer to [1] for details.

*MSC 2010*: 57Q15, 57R05.

*Keywords*: Combinatorial manifold; Tight triangulation; Strongly minimal triangulation.

---

For illustration purposes we discuss a single example of a tight and minimal triangulation of a handlebody. For details see [1].

Let  $(d, k, n) = (3, 2, 49)$ , which we denote by  $M_{k,i}^{d+1} = M_{2,1}^4$  ( $d$  dimension of the boundary of the handlebody,  $k$  number of layers of the underlying dual graph,  $n$  number of vertices). For this example, we have  $m$ -vector  $(m_0, m_1, m_2) = (41, 20, 1)$ , and treetypes:

$$\begin{aligned}\Delta(\sigma_1, \tau_1) &= \{(1, 4), (3, 2), (3, 4), (4, 2), (4, 3), (4, 4)\}, \\ \Delta(\sigma_2, \tau_2) &= \{(1, 3), (2, 3), (2, 4), (4, 1), (4, 3), (4, 4)\},\end{aligned}$$

where  $\mathcal{D} = \{(\sigma_1, \tau_1), (\sigma_2, \tau_2)\}$  is the 2-deck of permutations of  $\{0, 1, 2, 3\}$ . It can be seen that we must have

$$\sigma_1 = (1, 2, 0, 3), \tau_1 = (1, 0, 3, 2); \sigma_2 = (1, 0, 2, 3), \tau_2 = (0, 2, 1, 3).$$

Orbit representatives of the facets of  $M_{2,1}^4 = \mathcal{K}(G(3, 2; 41, 20, 1), \mathcal{DT})$  under the group action of  $\mathbb{Z}_{49} = \langle (0, 1, \dots, 48) \rangle$  are given by:

$$\begin{aligned}\langle 0, 1, 2, 3, 4 \rangle, \langle 0, 1, 3, 4, 31 \rangle, \langle 0, 1, 28, 37, 46 \rangle, \langle 0, 4, 11, 31, 40 \rangle, \langle 0, 9, 18, 29, 38 \rangle, \\ \langle 0, 6, 15, 24, 41 \rangle, \langle 0, 6, 16, 24, 41 \rangle, \langle 0, 8, 16, 24, 32 \rangle, \langle 0, 5, 11, 20, 29 \rangle.\end{aligned}$$

Below we list  $m$ -vectors and permutations (and in selected cases also treetypes and orbit representatives under the transitive cyclic group action) of the corresponding bounded neighborly members  $M_{k,\ell}^{d+1} \in \overline{\mathcal{K}}(d+1)$  for  $3 \leq d \leq 5$ , obtained by an implementation of the algorithm described in [1]. These have closed tight manifolds  $\partial M_{k,\ell}^{d+1} \in \mathcal{K}(d)$  as boundary.

The manifolds  $M_{1,i}^4$ ,  $1 \leq i \leq 4$ ,  $M_{1,j}^5$ ,  $1 \leq j \leq 16$ , and  $M_{1,\ell}^6$ ,  $1 \leq \ell \leq 64$ , from [1] belong to the infinite family of tight manifolds described in [1] and are thus not explicitly listed.

Table 1: 4-dimensional handlebodies with  $k = 1$

|             |                                                                                                                                                                                              |
|-------------|----------------------------------------------------------------------------------------------------------------------------------------------------------------------------------------------|
| $M_{1,5}^4$ | $m$ -vector: (12, 1)                                                                                                                                                                         |
| Perms.:     | $\sigma_1 = (2, 0, 1, 3), \quad \tau_1 = (1, 2, 0, 3)$                                                                                                                                       |
| Treetypes:  | $\Delta(\sigma_1, \tau_1) = \{(1, 2), (1, 4), (3, 4), (4, 1), (4, 2), (4, 4)\}$                                                                                                              |
| Orb. reps.: | $\langle 0, 1, 2, 3, 4 \rangle, \quad \langle 0, 1, 3, 4, 19 \rangle, \quad \langle 0, 1, 4, 19, 24 \rangle, \quad \langle 0, 4, 12, 19, 24 \rangle, \quad \langle 0, 5, 10, 17, 22 \rangle$ |
| $M_{1,6}^4$ | $m$ -vector: (12, 1)                                                                                                                                                                         |
| Perms.:     | $\sigma_1 = (2, 0, 3, 1), \quad \tau_1 = (1, 2, 0, 3)$                                                                                                                                       |
| Treetypes:  | $\Delta(\sigma_1, \tau_1) = \{(1, 2), (1, 4), (3, 1), (3, 2), (3, 4), (4, 4)\}$                                                                                                              |
| Orb. reps.: | $\langle 0, 1, 2, 3, 4 \rangle, \quad \langle 0, 1, 3, 4, 19 \rangle, \quad \langle 0, 1, 3, 19, 24 \rangle, \quad \langle 0, 3, 12, 19, 24 \rangle, \quad \langle 0, 5, 10, 17, 22 \rangle$ |

Table 2: 4-dimensional handlebodies with  $k = 2$

|             |                                                                                                                                                                                                                                                                                                                                                              |
|-------------|--------------------------------------------------------------------------------------------------------------------------------------------------------------------------------------------------------------------------------------------------------------------------------------------------------------------------------------------------------------|
| $M_{2,1}^4$ | $m$ -vector: (41, 20, 1)                                                                                                                                                                                                                                                                                                                                     |
| Perms.:     | $\sigma_2 = (1, 0, 2, 3), \quad \tau_2 = (0, 2, 1, 3);$<br>$\sigma_1 = (1, 2, 0, 3), \quad \tau_1 = (1, 0, 3, 2)$                                                                                                                                                                                                                                            |
| Treetypes:  | $\Delta(\sigma_2, \tau_2) = \{(1, 4), (3, 2), (3, 4), (4, 2), (4, 3), (4, 4)\},$<br>$\Delta(\sigma_1, \tau_1) = \{(1, 3), (2, 3), (2, 4), (4, 1), (4, 3), (4, 4)\}$                                                                                                                                                                                          |
| Orb. reps.: | $\langle 0, 1, 2, 3, 4 \rangle, \quad \langle 0, 1, 3, 4, 31 \rangle, \quad \langle 0, 1, 28, 37, 46 \rangle, \quad \langle 0, 4, 11, 31, 40 \rangle, \quad \langle 0, 9, 18, 29, 38 \rangle,$<br>$\langle 0, 6, 15, 24, 41 \rangle, \quad \langle 0, 6, 16, 24, 41 \rangle, \quad \langle 0, 8, 16, 24, 32 \rangle, \quad \langle 0, 5, 11, 20, 29 \rangle$ |

Table 3: 4-dimensional handlebodies with  $k = 3$

|             |                                                                                                                                                                                                                                                                                                                                                                                                                                                                                                                                 |
|-------------|---------------------------------------------------------------------------------------------------------------------------------------------------------------------------------------------------------------------------------------------------------------------------------------------------------------------------------------------------------------------------------------------------------------------------------------------------------------------------------------------------------------------------------|
| $M_{3,1}^4$ | $m$ -vector: (64, 25, 8, 1)                                                                                                                                                                                                                                                                                                                                                                                                                                                                                                     |
| Perms.:     | $\sigma_3 = (0, 2, 3, 1), \quad \tau_3 = (0, 3, 2, 1);$<br>$\sigma_2 = (3, 2, 0, 1), \quad \tau_2 = (3, 2, 0, 1);$<br>$\sigma_1 = (1, 0, 2, 3), \quad \tau_1 = (3, 1, 0, 2)$                                                                                                                                                                                                                                                                                                                                                    |
| Treetypes:  | $\Delta(\sigma_3, \tau_3) = \{(2, 2), (2, 3), (3, 2), (3, 3), (3, 4), (4, 2)\},$<br>$\Delta(\sigma_2, \tau_2) = \{(1, 1), (1, 2), (1, 4), (2, 1), (2, 2), (4, 1)\},$<br>$\Delta(\sigma_1, \tau_1) = \{(1, 1), (3, 1), (3, 4), (4, 1), (4, 2), (4, 4)\}$                                                                                                                                                                                                                                                                         |
| Orb. reps.: | $\langle 0, 1, 2, 3, 4 \rangle, \quad \langle 0, 1, 2, 14, 67 \rangle, \quad \langle 0, 1, 14, 22, 67 \rangle, \quad \langle 0, 3, 16, 24, 32 \rangle, \quad \langle 0, 6, 25, 31, 50 \rangle,$<br>$\langle 0, 5, 11, 30, 36 \rangle, \quad \langle 0, 5, 11, 36, 54 \rangle, \quad \langle 0, 8, 16, 24, 32 \rangle, \quad \langle 0, 7, 44, 52, 60 \rangle, \quad \langle 0, 8, 16, 25, 50 \rangle,$<br>$\langle 0, 6, 25, 44, 52 \rangle, \quad \langle 0, 5, 10, 41, 59 \rangle, \quad \langle 0, 5, 10, 15, 20 \rangle$    |
| $M_{3,2}^4$ | $m$ -vector: (62, 56, 11, 1)                                                                                                                                                                                                                                                                                                                                                                                                                                                                                                    |
| Perms.:     | $\sigma_3 = (0, 3, 1, 2), \quad \tau_3 = (1, 3, 0, 2);$<br>$\sigma_2 = (0, 2, 3, 1), \quad \tau_2 = (3, 1, 0, 2);$<br>$\sigma_1 = (3, 0, 1, 2), \quad \tau_1 = (3, 0, 2, 1)$                                                                                                                                                                                                                                                                                                                                                    |
| Treetypes:  | $\Delta(\sigma_3, \tau_3) = \{(2, 1), (2, 2), (2, 4), (3, 2), (4, 2), (4, 4)\},$<br>$\Delta(\sigma_2, \tau_2) = \{(2, 1), (2, 4), (3, 1), (3, 2), (3, 4), (4, 1)\},$<br>$\Delta(\sigma_1, \tau_1) = \{(1, 1), (1, 3), (1, 4), (3, 1), (4, 1), (4, 3)\}$                                                                                                                                                                                                                                                                         |
| Orb. reps.: | $\langle 0, 1, 2, 3, 4 \rangle, \quad \langle 0, 1, 2, 20, 67 \rangle, \quad \langle 0, 2, 4, 22, 44 \rangle, \quad \langle 0, 2, 11, 22, 44 \rangle, \quad \langle 0, 11, 22, 33, 44 \rangle,$<br>$\langle 0, 5, 16, 39, 52 \rangle, \quad \langle 0, 13, 26, 39, 52 \rangle, \quad \langle 0, 6, 13, 30, 43 \rangle, \quad \langle 0, 10, 23, 36, 53 \rangle, \quad \langle 0, 6, 13, 30, 61 \rangle,$<br>$\langle 0, 11, 22, 34, 47 \rangle, \quad \langle 0, 7, 14, 21, 28 \rangle, \quad \langle 0, 6, 13, 54, 61 \rangle$ |

continued on next page –

Table 3 – continued from previous page

|              |                                                                                    |
|--------------|------------------------------------------------------------------------------------|
| $M_{3,3}^4$  | $m$ -vector: (63, 11, 16, 1)                                                       |
| Perms.:      | (0, 3, 2, 1), (2, 1, 0, 3); (0, 1, 2, 3), (0, 3, 2, 1); (2, 3, 0, 1), (3, 0, 1, 2) |
| $M_{3,4}^4$  | $m$ -vector: (63, 11, 16, 1)                                                       |
| Perms.:      | (0, 3, 2, 1), (2, 1, 0, 3); (0, 1, 2, 3), (0, 3, 2, 1); (3, 2, 0, 1), (3, 0, 1, 2) |
| $M_{3,5}^4$  | $m$ -vector: (63, 11, 16, 1)                                                       |
| Perms.:      | (0, 3, 2, 1), (1, 2, 0, 3); (0, 1, 2, 3), (0, 3, 2, 1); (3, 1, 0, 2), (3, 2, 0, 1) |
| $M_{3,6}^4$  | $m$ -vector: (63, 11, 16, 1)                                                       |
| Perms.:      | (0, 3, 2, 1), (1, 2, 0, 3); (0, 1, 2, 3), (0, 3, 2, 1); (1, 3, 0, 2), (3, 2, 0, 1) |
| $M_{3,7}^4$  | $m$ -vector: (11, 37, 39, 1)                                                       |
| Perms.:      | (0, 2, 3, 1), (0, 2, 1, 3); (1, 0, 2, 3), (1, 2, 0, 3); (0, 2, 1, 3), (0, 3, 2, 1) |
| $M_{3,8}^4$  | $m$ -vector: (40, 14, 44, 1)                                                       |
| Perms.:      | (0, 3, 1, 2), (0, 2, 3, 1); (2, 0, 3, 1), (3, 0, 1, 2); (2, 1, 0, 3), (2, 0, 3, 1) |
| $M_{3,9}^4$  | $m$ -vector: (44, 5, 55, 1)                                                        |
| Perms.:      | (1, 3, 0, 2), (1, 2, 0, 3); (0, 2, 3, 1), (3, 1, 0, 2); (0, 1, 2, 3), (3, 0, 1, 2) |
| $M_{3,10}^4$ | $m$ -vector: (63, 5, 55, 1)                                                        |
| Perms.:      | (0, 2, 1, 3), (0, 3, 1, 2); (1, 3, 0, 2), (3, 0, 1, 2); (2, 3, 0, 1), (1, 2, 0, 3) |
| $M_{3,11}^4$ | $m$ -vector: (63, 5, 55, 1)                                                        |
| Perms.:      | (1, 2, 0, 3), (0, 3, 1, 2); (2, 0, 3, 1), (3, 1, 0, 2); (0, 1, 2, 3), (3, 0, 2, 1) |
| $M_{3,12}^4$ | $m$ -vector: (63, 5, 55, 1)                                                        |
| Perms.:      | (1, 3, 0, 2), (1, 3, 0, 2); (2, 0, 3, 1), (3, 1, 0, 2); (1, 0, 2, 3), (2, 0, 3, 1) |
| $M_{3,13}^4$ | $m$ -vector: (60, 19, 64, 1)                                                       |
| Perms.:      | (0, 1, 3, 2), (1, 2, 0, 3); (0, 3, 1, 2), (3, 2, 0, 1); (2, 0, 1, 3), (2, 3, 0, 1) |
| $M_{3,14}^4$ | $m$ -vector: (60, 19, 64, 1)                                                       |
| Perms.:      | (2, 0, 3, 1), (1, 2, 0, 3); (0, 2, 3, 1), (3, 1, 0, 2); (3, 0, 1, 2), (1, 3, 0, 2) |
| $M_{3,15}^4$ | $m$ -vector: (60, 19, 64, 1)                                                       |
| Perms.:      | (1, 0, 3, 2), (1, 3, 0, 2); (0, 3, 2, 1), (3, 1, 0, 2); (2, 0, 1, 3), (2, 3, 0, 1) |

Table 4: 4-dimensional handlebodies with  $k = 4$ 

|             |                                                                                                                                                                                                                                                                                                                                                                                                                                                                                                                                                                                                                                                                                               |
|-------------|-----------------------------------------------------------------------------------------------------------------------------------------------------------------------------------------------------------------------------------------------------------------------------------------------------------------------------------------------------------------------------------------------------------------------------------------------------------------------------------------------------------------------------------------------------------------------------------------------------------------------------------------------------------------------------------------------|
| $M_{4,1}^4$ | $m$ -vector: (36, 78, 20, 7, 1)                                                                                                                                                                                                                                                                                                                                                                                                                                                                                                                                                                                                                                                               |
| Perms.:     | $\sigma_4 = (3, 0, 1, 2), \quad \tau_4 = (1, 2, 0, 3);$<br>$\sigma_3 = (0, 2, 1, 3), \quad \tau_3 = (1, 0, 3, 2);$<br>$\sigma_2 = (0, 3, 2, 1), \quad \tau_2 = (2, 0, 1, 3);$<br>$\sigma_1 = (2, 3, 0, 1), \quad \tau_1 = (2, 0, 3, 1)$                                                                                                                                                                                                                                                                                                                                                                                                                                                       |
| Treotypes:  | $\Delta(\sigma_4, \tau_4) = \{(1, 1), (1, 2), (1, 4), (3, 4), (4, 2), (4, 4)\},$<br>$\Delta(\sigma_3, \tau_3) = \{(2, 3), (2, 4), (3, 3), (4, 1), (4, 3), (4, 4)\},$<br>$\Delta(\sigma_2, \tau_2) = \{(2, 1), (2, 3), (2, 4), (3, 1), (3, 4), (4, 4)\},$<br>$\Delta(\sigma_1, \tau_1) = \{(1, 1), (1, 3), (2, 1), (2, 3), (2, 4), (4, 3)\}$                                                                                                                                                                                                                                                                                                                                                   |
| Orb. reps.: | $\langle 0, 1, 2, 3, 4 \rangle, \quad \langle 0, 1, 3, 4, 28 \rangle, \quad \langle 0, 1, 4, 14, 28 \rangle, \quad \langle 0, 1, 7, 14, 28 \rangle, \quad \langle 0, 7, 14, 21, 28 \rangle,$<br>$\langle 0, 7, 14, 46, 75 \rangle, \quad \langle 0, 9, 23, 37, 69 \rangle, \quad \langle 0, 12, 34, 53, 70 \rangle, \quad \langle 0, 17, 34, 53, 70 \rangle, \quad \langle 0, 11, 22, 41, 58 \rangle,$<br>$\langle 0, 11, 22, 41, 67 \rangle, \quad \langle 0, 8, 40, 60, 69 \rangle, \quad \langle 0, 9, 29, 49, 69 \rangle, \quad \langle 0, 5, 16, 38, 49 \rangle, \quad \langle 0, 5, 20, 38, 49 \rangle,$<br>$\langle 0, 5, 20, 40, 49 \rangle, \quad \langle 0, 11, 22, 33, 44 \rangle$ |

continued on next page –

Table 4 – continued from previous page

|              |                                                                                                                                                                                                                                                                                                                                                                                                                                                                                                                                                                                                                                                                                               |
|--------------|-----------------------------------------------------------------------------------------------------------------------------------------------------------------------------------------------------------------------------------------------------------------------------------------------------------------------------------------------------------------------------------------------------------------------------------------------------------------------------------------------------------------------------------------------------------------------------------------------------------------------------------------------------------------------------------------------|
| $M_{4,2}^4$  | $m$ -vector: (48, 27, 83, 10, 1)                                                                                                                                                                                                                                                                                                                                                                                                                                                                                                                                                                                                                                                              |
| Perms.:      | $\sigma_4 = (3, 2, 0, 1), \quad \tau_4 = (1, 0, 2, 3);$<br>$\sigma_3 = (0, 3, 1, 2), \quad \tau_3 = (1, 3, 0, 2);$<br>$\sigma_2 = (0, 2, 1, 3), \quad \tau_2 = (0, 3, 1, 2);$<br>$\sigma_1 = (2, 0, 3, 1), \quad \tau_1 = (2, 1, 0, 3)$                                                                                                                                                                                                                                                                                                                                                                                                                                                       |
| Treotypes:   | $\Delta(\sigma_4, \tau_4) = \{(1, 1), (1, 3), (1, 4), (2, 3), (2, 4), (4, 4)\},$<br>$\Delta(\sigma_3, \tau_3) = \{(2, 1), (2, 2), (2, 4), (3, 2), (4, 2), (4, 4)\},$<br>$\Delta(\sigma_2, \tau_2) = \{(2, 2), (2, 4), (3, 2), (4, 2), (4, 3), (4, 4)\},$<br>$\Delta(\sigma_1, \tau_1) = \{(1, 1), (1, 4), (3, 1), (3, 2), (3, 4), (4, 4)\}$                                                                                                                                                                                                                                                                                                                                                   |
| Orb. reps.:  | $\langle 0, 1, 2, 3, 4 \rangle, \quad \langle 0, 1, 2, 4, 40 \rangle, \quad \langle 0, 1, 2, 30, 40 \rangle, \quad \langle 0, 1, 10, 30, 40 \rangle, \quad \langle 0, 7, 14, 48, 55 \rangle,$<br>$\langle 0, 7, 14, 48, 81 \rangle, \quad \langle 0, 10, 20, 30, 40 \rangle, \quad \langle 0, 5, 13, 67, 75 \rangle, \quad \langle 0, 8, 22, 35, 56 \rangle, \quad \langle 0, 8, 27, 35, 62 \rangle,$<br>$\langle 0, 11, 23, 35, 54 \rangle, \quad \langle 0, 8, 27, 62, 73 \rangle, \quad \langle 0, 10, 20, 57, 69 \rangle, \quad \langle 0, 12, 24, 44, 64 \rangle, \quad \langle 0, 6, 12, 32, 77 \rangle,$<br>$\langle 0, 6, 12, 24, 78 \rangle, \quad \langle 0, 6, 12, 18, 24 \rangle$ |
| $M_{4,3}^4$  | $m$ -vector: (17, 76, 69, 12, 1)                                                                                                                                                                                                                                                                                                                                                                                                                                                                                                                                                                                                                                                              |
| Perms.:      | (3, 2, 0, 1), (2, 1, 0, 3); (0, 3, 2, 1), (0, 1, 3, 2); (2, 1, 0, 3), (1, 3, 0, 2); (2, 0, 3, 1), (2, 1, 0, 3)                                                                                                                                                                                                                                                                                                                                                                                                                                                                                                                                                                                |
| $M_{4,4}^4$  | $m$ -vector: (7, 53, 74, 13, 1)                                                                                                                                                                                                                                                                                                                                                                                                                                                                                                                                                                                                                                                               |
| Perms.:      | (2, 1, 0, 3), (0, 3, 2, 1); (3, 1, 0, 2), (0, 1, 3, 2); (1, 0, 3, 2), (1, 3, 0, 2); (0, 1, 3, 2), (0, 2, 1, 3)                                                                                                                                                                                                                                                                                                                                                                                                                                                                                                                                                                                |
| $M_{4,5}^4$  | $m$ -vector: (7, 53, 74, 13, 1)                                                                                                                                                                                                                                                                                                                                                                                                                                                                                                                                                                                                                                                               |
| Perms.:      | (2, 1, 0, 3), (0, 3, 1, 2); (3, 1, 0, 2), (0, 1, 3, 2); (1, 0, 3, 2), (1, 3, 0, 2); (0, 1, 3, 2), (0, 2, 1, 3)                                                                                                                                                                                                                                                                                                                                                                                                                                                                                                                                                                                |
| $M_{4,6}^4$  | $m$ -vector: (6, 74, 35, 14, 1)                                                                                                                                                                                                                                                                                                                                                                                                                                                                                                                                                                                                                                                               |
| Perms.:      | (1, 0, 3, 2), (2, 1, 0, 3); (0, 1, 2, 3), (2, 0, 1, 3); (0, 1, 3, 2), (1, 2, 0, 3); (2, 0, 3, 1), (0, 3, 1, 2)                                                                                                                                                                                                                                                                                                                                                                                                                                                                                                                                                                                |
| $M_{4,7}^4$  | $m$ -vector: (6, 74, 35, 14, 1)                                                                                                                                                                                                                                                                                                                                                                                                                                                                                                                                                                                                                                                               |
| Perms.:      | (1, 0, 3, 2), (2, 1, 0, 3); (0, 1, 3, 2), (1, 0, 2, 3); (0, 1, 3, 2), (1, 2, 0, 3); (3, 0, 2, 1), (1, 3, 0, 2)                                                                                                                                                                                                                                                                                                                                                                                                                                                                                                                                                                                |
| $M_{4,8}^4$  | $m$ -vector: (6, 74, 35, 14, 1)                                                                                                                                                                                                                                                                                                                                                                                                                                                                                                                                                                                                                                                               |
| Perms.:      | (1, 0, 3, 2), (2, 1, 0, 3); (0, 2, 1, 3), (2, 0, 1, 3); (0, 1, 3, 2), (1, 2, 0, 3); (2, 0, 3, 1), (0, 3, 1, 2)                                                                                                                                                                                                                                                                                                                                                                                                                                                                                                                                                                                |
| $M_{4,9}^4$  | $m$ -vector: (17, 73, 42, 15, 1)                                                                                                                                                                                                                                                                                                                                                                                                                                                                                                                                                                                                                                                              |
| Perms.:      | (1, 2, 0, 3), (3, 2, 0, 1); (0, 2, 1, 3), (1, 3, 0, 2); (1, 0, 3, 2), (3, 2, 0, 1); (0, 1, 2, 3), (1, 3, 0, 2)                                                                                                                                                                                                                                                                                                                                                                                                                                                                                                                                                                                |
| $M_{4,10}^4$ | $m$ -vector: (17, 73, 42, 15, 1)                                                                                                                                                                                                                                                                                                                                                                                                                                                                                                                                                                                                                                                              |
| Perms.:      | (1, 2, 0, 3), (3, 2, 0, 1); (2, 0, 1, 3), (2, 3, 0, 1); (1, 0, 2, 3), (3, 1, 0, 2); (0, 2, 1, 3), (2, 3, 0, 1)                                                                                                                                                                                                                                                                                                                                                                                                                                                                                                                                                                                |
| $M_{4,11}^4$ | $m$ -vector: (12, 40, 57, 15, 1)                                                                                                                                                                                                                                                                                                                                                                                                                                                                                                                                                                                                                                                              |
| Perms.:      | (1, 2, 0, 3), (3, 2, 0, 1); (0, 3, 1, 2), (1, 0, 2, 3); (0, 3, 1, 2), (0, 1, 3, 2); (2, 0, 1, 3), (0, 2, 1, 3)                                                                                                                                                                                                                                                                                                                                                                                                                                                                                                                                                                                |
| $M_{4,12}^4$ | $m$ -vector: (39, 74, 83, 19, 1)                                                                                                                                                                                                                                                                                                                                                                                                                                                                                                                                                                                                                                                              |
| Perms.:      | (3, 0, 2, 1), (0, 1, 2, 3); (3, 0, 2, 1), (3, 1, 0, 2); (0, 1, 2, 3), (1, 0, 2, 3); (0, 1, 3, 2), (3, 2, 0, 1)                                                                                                                                                                                                                                                                                                                                                                                                                                                                                                                                                                                |
| $M_{4,13}^4$ | $m$ -vector: (39, 74, 83, 19, 1)                                                                                                                                                                                                                                                                                                                                                                                                                                                                                                                                                                                                                                                              |
| Perms.:      | (3, 0, 2, 1), (0, 2, 1, 3); (3, 0, 2, 1), (3, 1, 0, 2); (0, 1, 2, 3), (1, 0, 2, 3); (0, 1, 3, 2), (3, 2, 0, 1)                                                                                                                                                                                                                                                                                                                                                                                                                                                                                                                                                                                |
| $M_{4,14}^4$ | $m$ -vector: (57, 28, 34, 20, 1)                                                                                                                                                                                                                                                                                                                                                                                                                                                                                                                                                                                                                                                              |
| Perms.:      | (0, 3, 1, 2), (3, 2, 0, 1); (3, 0, 1, 2), (2, 3, 0, 1); (0, 1, 2, 3), (2, 0, 1, 3); (2, 3, 0, 1), (0, 1, 3, 2)                                                                                                                                                                                                                                                                                                                                                                                                                                                                                                                                                                                |
| $M_{4,15}^4$ | $m$ -vector: (78, 8, 48, 21, 1)                                                                                                                                                                                                                                                                                                                                                                                                                                                                                                                                                                                                                                                               |
| Perms.:      | (2, 1, 0, 3), (2, 0, 3, 1); (0, 1, 2, 3), (3, 1, 0, 2); (0, 1, 3, 2), (0, 1, 2, 3); (1, 2, 0, 3), (1, 2, 0, 3)                                                                                                                                                                                                                                                                                                                                                                                                                                                                                                                                                                                |
| $M_{4,16}^4$ | $m$ -vector: (8, 78, 48, 21, 1)                                                                                                                                                                                                                                                                                                                                                                                                                                                                                                                                                                                                                                                               |
| Perms.:      | (1, 0, 2, 3), (3, 2, 0, 1); (0, 3, 1, 2), (3, 1, 0, 2); (1, 0, 3, 2), (3, 1, 0, 2); (2, 0, 1, 3), (1, 3, 0, 2)                                                                                                                                                                                                                                                                                                                                                                                                                                                                                                                                                                                |
| $M_{4,17}^4$ | $m$ -vector: (51, 37, 20, 24, 1)                                                                                                                                                                                                                                                                                                                                                                                                                                                                                                                                                                                                                                                              |
| Perms.:      | (2, 3, 0, 1), (0, 3, 2, 1); (1, 3, 0, 2), (1, 0, 2, 3); (2, 1, 0, 3), (0, 3, 1, 2); (3, 2, 0, 1), (3, 0, 2, 1)                                                                                                                                                                                                                                                                                                                                                                                                                                                                                                                                                                                |
| $M_{4,18}^4$ | $m$ -vector: (51, 37, 20, 24, 1)                                                                                                                                                                                                                                                                                                                                                                                                                                                                                                                                                                                                                                                              |
| Perms.:      | (2, 3, 0, 1), (0, 3, 2, 1); (2, 3, 0, 1), (1, 0, 2, 3); (2, 1, 0, 3), (0, 3, 1, 2); (3, 2, 0, 1), (3, 0, 2, 1)                                                                                                                                                                                                                                                                                                                                                                                                                                                                                                                                                                                |

continued on next page –

Table 4 – continued from previous page

|              |                                                                                                                |
|--------------|----------------------------------------------------------------------------------------------------------------|
| $M_{4,19}^4$ | $m$ -vector: (62, 77, 34, 26, 1)                                                                               |
| Perms.:      | (3, 0, 2, 1), (3, 2, 0, 1); (0, 3, 2, 1), (0, 2, 1, 3); (2, 0, 1, 3), (2, 1, 0, 3); (1, 0, 3, 2), (1, 0, 3, 2) |
| $M_{4,20}^4$ | $m$ -vector: (69, 55, 11, 27, 1)                                                                               |
| Perms.:      | (3, 0, 1, 2), (1, 3, 0, 2); (3, 0, 2, 1), (1, 2, 0, 3); (3, 0, 1, 2), (0, 3, 2, 1); (3, 2, 0, 1), (2, 3, 0, 1) |
| $M_{4,21}^4$ | $m$ -vector: (69, 55, 11, 27, 1)                                                                               |
| Perms.:      | (3, 0, 1, 2), (1, 3, 0, 2); (3, 0, 2, 1), (1, 2, 0, 3); (3, 0, 1, 2), (0, 2, 3, 1); (2, 3, 0, 1), (2, 3, 0, 1) |
| $M_{4,22}^4$ | $m$ -vector: (16, 49, 15, 28, 1)                                                                               |
| Perms.:      | (0, 3, 2, 1), (0, 3, 2, 1); (2, 0, 3, 1), (2, 0, 3, 1); (0, 2, 1, 3), (2, 1, 0, 3); (0, 1, 3, 2), (0, 2, 1, 3) |
| $M_{4,23}^4$ | $m$ -vector: (16, 49, 15, 28, 1)                                                                               |
| Perms.:      | (1, 3, 0, 2), (0, 3, 1, 2); (1, 0, 3, 2), (3, 0, 2, 1); (0, 1, 2, 3), (1, 2, 0, 3); (1, 0, 3, 2), (0, 3, 1, 2) |
| $M_{4,24}^4$ | $m$ -vector: (16, 49, 15, 28, 1)                                                                               |
| Perms.:      | (1, 3, 0, 2), (0, 2, 1, 3); (2, 0, 3, 1), (3, 0, 2, 1); (0, 1, 2, 3), (1, 2, 0, 3); (0, 1, 3, 2), (0, 2, 1, 3) |
| $M_{4,25}^4$ | $m$ -vector: (16, 49, 15, 28, 1)                                                                               |
| Perms.:      | (2, 3, 0, 1), (0, 2, 1, 3); (1, 0, 3, 2), (3, 0, 1, 2); (0, 1, 2, 3), (1, 2, 0, 3); (1, 0, 3, 2), (0, 3, 1, 2) |
| $M_{4,26}^4$ | $m$ -vector: (69, 33, 27, 32, 1)                                                                               |
| Perms.:      | (3, 2, 0, 1), (3, 1, 0, 2); (3, 0, 2, 1), (1, 3, 0, 2); (0, 3, 2, 1), (3, 0, 2, 1); (3, 1, 0, 2), (1, 3, 0, 2) |
| $M_{4,27}^4$ | $m$ -vector: (69, 33, 27, 32, 1)                                                                               |
| Perms.:      | (3, 2, 0, 1), (3, 1, 0, 2); (3, 0, 1, 2), (2, 3, 0, 1); (0, 3, 2, 1), (3, 0, 2, 1); (3, 1, 0, 2), (1, 3, 0, 2) |
| $M_{4,28}^4$ | $m$ -vector: (54, 83, 7, 33, 1)                                                                                |
| Perms.:      | (3, 2, 0, 1), (1, 0, 2, 3); (2, 1, 0, 3), (3, 0, 1, 2); (2, 1, 0, 3), (3, 1, 0, 2); (3, 0, 1, 2), (3, 1, 0, 2) |
| $M_{4,29}^4$ | $m$ -vector: (19, 52, 18, 33, 1)                                                                               |
| Perms.:      | (1, 3, 0, 2), (0, 1, 3, 2); (1, 0, 2, 3), (0, 2, 3, 1); (3, 2, 0, 1), (3, 0, 2, 1); (3, 2, 0, 1), (0, 1, 3, 2) |
| $M_{4,30}^4$ | $m$ -vector: (6, 33, 21, 41, 1)                                                                                |
| Perms.:      | (0, 2, 3, 1), (1, 0, 3, 2); (0, 2, 3, 1), (3, 2, 0, 1); (3, 0, 2, 1), (0, 1, 3, 2); (2, 1, 0, 3), (3, 0, 1, 2) |
| $M_{4,31}^4$ | $m$ -vector: (40, 81, 15, 42, 1)                                                                               |
| Perms.:      | (3, 2, 0, 1), (1, 0, 3, 2); (0, 1, 3, 2), (3, 1, 0, 2); (0, 3, 1, 2), (2, 3, 0, 1); (1, 0, 2, 3), (1, 0, 3, 2) |
| $M_{4,32}^4$ | $m$ -vector: (20, 18, 61, 55, 1)                                                                               |
| Perms.:      | (2, 0, 3, 1), (1, 0, 2, 3); (0, 1, 3, 2), (2, 1, 0, 3); (3, 0, 2, 1), (0, 3, 1, 2); (1, 0, 2, 3), (0, 1, 2, 3) |
| $M_{4,33}^4$ | $m$ -vector: (20, 18, 61, 55, 1)                                                                               |
| Perms.:      | (2, 0, 3, 1), (1, 0, 2, 3); (0, 1, 3, 2), (2, 1, 0, 3); (3, 0, 1, 2), (0, 3, 1, 2); (2, 0, 1, 3), (0, 2, 1, 3) |
| $M_{4,34}^4$ | $m$ -vector: (63, 75, 17, 69, 1)                                                                               |
| Perms.:      | (0, 1, 3, 2), (3, 1, 0, 2); (0, 2, 1, 3), (3, 1, 0, 2); (3, 0, 1, 2), (2, 1, 0, 3); (0, 2, 3, 1), (0, 1, 2, 3) |
| $M_{4,35}^4$ | $m$ -vector: (63, 75, 17, 69, 1)                                                                               |
| Perms.:      | (0, 1, 3, 2), (3, 1, 0, 2); (0, 2, 1, 3), (3, 1, 0, 2); (3, 0, 1, 2), (1, 2, 0, 3); (0, 2, 3, 1), (0, 1, 2, 3) |
| $M_{4,36}^4$ | $m$ -vector: (63, 75, 17, 69, 1)                                                                               |
| Perms.:      | (0, 2, 3, 1), (2, 1, 0, 3); (0, 2, 1, 3), (3, 1, 0, 2); (3, 0, 2, 1), (2, 1, 0, 3); (0, 2, 3, 1), (0, 1, 2, 3) |
| $M_{4,37}^4$ | $m$ -vector: (63, 75, 17, 69, 1)                                                                               |
| Perms.:      | (0, 2, 3, 1), (2, 1, 0, 3); (0, 2, 1, 3), (3, 1, 0, 2); (3, 0, 2, 1), (1, 2, 0, 3); (0, 3, 2, 1), (0, 1, 2, 3) |
| $M_{4,38}^4$ | $m$ -vector: (63, 75, 17, 69, 1)                                                                               |
| Perms.:      | (1, 0, 3, 2), (1, 3, 0, 2); (0, 2, 1, 3), (3, 1, 0, 2); (1, 0, 3, 2), (3, 1, 0, 2); (0, 2, 3, 1), (1, 0, 3, 2) |
| $M_{4,39}^4$ | $m$ -vector: (47, 32, 72, 74, 1)                                                                               |

continued on next page –

Table 4 – continued from previous page

|              |                                                                                                                |
|--------------|----------------------------------------------------------------------------------------------------------------|
| Perms.:      | (3, 0, 2, 1), (0, 1, 3, 2); (2, 0, 3, 1), (0, 2, 3, 1); (3, 1, 0, 2), (0, 1, 2, 3); (3, 2, 0, 1), (0, 1, 3, 2) |
| $M_{4,40}^4$ | $m$ -vector: (47, 32, 72, 74, 1)                                                                               |
| Perms.:      | (3, 0, 2, 1), (3, 1, 0, 2); (1, 0, 2, 3), (1, 0, 2, 3); (3, 1, 0, 2), (2, 0, 3, 1); (3, 2, 0, 1), (0, 1, 3, 2) |
| $M_{4,41}^4$ | $m$ -vector: (47, 32, 72, 74, 1)                                                                               |
| Perms.:      | (3, 0, 2, 1), (3, 1, 0, 2); (1, 0, 2, 3), (1, 0, 3, 2); (3, 1, 0, 2), (2, 0, 3, 1); (3, 2, 0, 1), (0, 1, 3, 2) |

Table 5: 4-dimensional handlebodies with  $k = 5$ 

|             |                                                                                                                                                                                                                                                                                                                                                                                                                                                                                                                                                                                                                                                                                                                                                                |
|-------------|----------------------------------------------------------------------------------------------------------------------------------------------------------------------------------------------------------------------------------------------------------------------------------------------------------------------------------------------------------------------------------------------------------------------------------------------------------------------------------------------------------------------------------------------------------------------------------------------------------------------------------------------------------------------------------------------------------------------------------------------------------------|
| $M_{5,1}^4$ | $m$ -vector: (91, 26, 86, 75, 8, 1)                                                                                                                                                                                                                                                                                                                                                                                                                                                                                                                                                                                                                                                                                                                            |
| Perms.:     | $\sigma_5 = (0, 3, 1, 2), \tau_5 = (1, 0, 2, 3);$<br>$\sigma_4 = (3, 2, 0, 1), \tau_4 = (1, 2, 0, 3);$<br>$\sigma_3 = (3, 0, 2, 1), \tau_3 = (1, 3, 0, 2);$<br>$\sigma_2 = (1, 0, 3, 2), \tau_2 = (3, 0, 2, 1);$<br>$\sigma_1 = (2, 3, 0, 1), \tau_1 = (3, 2, 0, 1)$                                                                                                                                                                                                                                                                                                                                                                                                                                                                                           |
| Tree-types: | $\Delta(\sigma_5, \tau_5) = \{(2, 1), (2, 3), (2, 4), (3, 4), (4, 3), (4, 4)\},$<br>$\Delta(\sigma_4, \tau_4) = \{(1, 1), (1, 2), (1, 4), (2, 2), (2, 4), (4, 4)\},$<br>$\Delta(\sigma_3, \tau_3) = \{(1, 1), (1, 2), (1, 4), (3, 2), (3, 4), (4, 2)\},$<br>$\Delta(\sigma_2, \tau_2) = \{(1, 1), (3, 1), (3, 3), (3, 4), (4, 1), (4, 3)\},$<br>$\Delta(\sigma_1, \tau_1) = \{(1, 1), (1, 2), (2, 1), (2, 2), (2, 4), (4, 1)\}$                                                                                                                                                                                                                                                                                                                                |
| Orb. reps.: | $\langle 0, 1, 2, 3, 4 \rangle, \langle 0, 1, 2, 30, 107 \rangle, \langle 0, 2, 4, 24, 32 \rangle, \langle 0, 2, 8, 24, 32 \rangle, \langle 0, 7, 17, 63, 75 \rangle,$<br>$\langle 0, 7, 34, 41, 75 \rangle, \langle 0, 7, 34, 41, 97 \rangle, \langle 0, 8, 16, 24, 32 \rangle, \langle 0, 8, 16, 32, 82 \rangle, \langle 0, 8, 16, 41, 82 \rangle,$<br>$\langle 0, 7, 34, 42, 75 \rangle, \langle 0, 9, 23, 61, 92 \rangle, \langle 0, 9, 23, 69, 92 \rangle, \langle 0, 17, 40, 63, 86 \rangle, \langle 0, 11, 34, 51, 97 \rangle,$<br>$\langle 0, 5, 31, 45, 83 \rangle, \langle 0, 18, 36, 62, 88 \rangle, \langle 0, 5, 31, 57, 83 \rangle, \langle 0, 5, 31, 57, 96 \rangle, \langle 0, 15, 36, 54, 72 \rangle,$<br>$\langle 0, 18, 36, 54, 72 \rangle$ |
| $M_{5,2}^4$ | $m$ -vector: (91, 26, 86, 75, 8, 1)                                                                                                                                                                                                                                                                                                                                                                                                                                                                                                                                                                                                                                                                                                                            |
| Perms.:     | $\sigma_5 = (0, 3, 1, 2), \tau_5 = (1, 0, 2, 3);$<br>$\sigma_4 = (3, 2, 0, 1), \tau_4 = (3, 2, 0, 1);$<br>$\sigma_3 = (3, 0, 2, 1), \tau_3 = (1, 3, 0, 2);$<br>$\sigma_2 = (1, 0, 3, 2), \tau_2 = (3, 0, 2, 1);$<br>$\sigma_1 = (2, 3, 0, 1), \tau_1 = (3, 2, 0, 1)$                                                                                                                                                                                                                                                                                                                                                                                                                                                                                           |
| Tree-types: | $\Delta(\sigma_5, \tau_5) = \{(2, 1), (2, 3), (2, 4), (3, 4), (4, 3), (4, 4)\},$<br>$\Delta(\sigma_4, \tau_4) = \{(1, 1), (1, 2), (1, 4), (2, 1), (2, 2), (4, 1)\},$<br>$\Delta(\sigma_3, \tau_3) = \{(1, 1), (1, 2), (1, 4), (3, 2), (3, 4), (4, 2)\},$<br>$\Delta(\sigma_2, \tau_2) = \{(1, 1), (3, 1), (3, 3), (3, 4), (4, 1), (4, 3)\},$<br>$\Delta(\sigma_1, \tau_1) = \{(1, 1), (1, 2), (2, 1), (2, 2), (2, 4), (4, 1)\}$                                                                                                                                                                                                                                                                                                                                |
| Orb. reps.: | $\langle 0, 1, 2, 3, 4 \rangle, \langle 0, 1, 2, 30, 107 \rangle, \langle 0, 2, 4, 24, 32 \rangle, \langle 0, 2, 8, 24, 32 \rangle, \langle 0, 7, 17, 63, 75 \rangle,$<br>$\langle 0, 7, 34, 41, 75 \rangle, \langle 0, 7, 34, 41, 97 \rangle, \langle 0, 8, 16, 24, 32 \rangle, \langle 0, 8, 16, 32, 75 \rangle, \langle 0, 8, 16, 41, 75 \rangle,$<br>$\langle 0, 7, 34, 42, 75 \rangle, \langle 0, 9, 23, 61, 92 \rangle, \langle 0, 9, 23, 69, 92 \rangle, \langle 0, 17, 40, 63, 86 \rangle, \langle 0, 11, 34, 51, 97 \rangle,$<br>$\langle 0, 5, 31, 45, 83 \rangle, \langle 0, 18, 36, 62, 88 \rangle, \langle 0, 5, 31, 57, 83 \rangle, \langle 0, 5, 31, 57, 96 \rangle, \langle 0, 15, 36, 54, 72 \rangle,$<br>$\langle 0, 18, 36, 54, 72 \rangle$ |
| $M_{5,3}^4$ | $m$ -vector: (77, 98, 31, 99, 9, 1)                                                                                                                                                                                                                                                                                                                                                                                                                                                                                                                                                                                                                                                                                                                            |
| Perms.:     | (3, 1, 0, 2), (0, 2, 3, 1); (3, 1, 0, 2), (0, 2, 3, 1); (2, 1, 0, 3), (3, 2, 0, 1); (2, 0, 3, 1), (2, 1, 0, 3); (3, 0, 1, 2), (2, 0, 3, 1)                                                                                                                                                                                                                                                                                                                                                                                                                                                                                                                                                                                                                     |
| $M_{5,4}^4$ | $m$ -vector: (97, 78, 34, 77, 10, 1)                                                                                                                                                                                                                                                                                                                                                                                                                                                                                                                                                                                                                                                                                                                           |
| Perms.:     | (2, 3, 0, 1), (3, 0, 2, 1); (2, 3, 0, 1), (3, 2, 0, 1); (1, 0, 2, 3), (3, 2, 0, 1); (3, 0, 1, 2), (2, 0, 3, 1); (2, 3, 0, 1), (1, 0, 2, 3)                                                                                                                                                                                                                                                                                                                                                                                                                                                                                                                                                                                                                     |
| $M_{5,5}^4$ | $m$ -vector: (97, 78, 34, 77, 10, 1)                                                                                                                                                                                                                                                                                                                                                                                                                                                                                                                                                                                                                                                                                                                           |
| Perms.:     | (2, 3, 0, 1), (3, 0, 1, 2); (3, 2, 0, 1), (3, 2, 0, 1); (1, 0, 2, 3), (3, 2, 0, 1); (3, 0, 1, 2), (2, 0, 3, 1); (2, 3, 0, 1), (1, 0, 2, 3)                                                                                                                                                                                                                                                                                                                                                                                                                                                                                                                                                                                                                     |
| $M_{5,6}^4$ | $m$ -vector: (102, 63, 61, 94, 11, 1)                                                                                                                                                                                                                                                                                                                                                                                                                                                                                                                                                                                                                                                                                                                          |
| Perms.:     | (3, 2, 0, 1), (1, 0, 2, 3); (0, 2, 1, 3), (2, 0, 1, 3); (0, 1, 2, 3), (1, 2, 0, 3); (1, 0, 2, 3), (0, 2, 3, 1); (3, 1, 0, 2), (3, 0, 1, 2)                                                                                                                                                                                                                                                                                                                                                                                                                                                                                                                                                                                                                     |
| $M_{5,7}^4$ | $m$ -vector: (103, 7, 92, 94, 11, 1)                                                                                                                                                                                                                                                                                                                                                                                                                                                                                                                                                                                                                                                                                                                           |
| Perms.:     | (3, 1, 0, 2), (1, 0, 2, 3); (0, 1, 2, 3), (3, 1, 0, 2); (2, 0, 1, 3), (0, 1, 2, 3); (1, 2, 0, 3), (0, 1, 3, 2); (3, 0, 1, 2), (0, 1, 3, 2)                                                                                                                                                                                                                                                                                                                                                                                                                                                                                                                                                                                                                     |
| $M_{5,8}^4$ | $m$ -vector: (103, 7, 92, 94, 11, 1)                                                                                                                                                                                                                                                                                                                                                                                                                                                                                                                                                                                                                                                                                                                           |
| Perms.:     | (3, 1, 0, 2), (1, 0, 2, 3); (0, 2, 1, 3), (2, 1, 0, 3); (2, 0, 1, 3), (0, 1, 2, 3); (1, 3, 0, 2), (0, 1, 3, 2); (3, 0, 1, 2), (0, 1, 3, 2)                                                                                                                                                                                                                                                                                                                                                                                                                                                                                                                                                                                                                     |

continued on next page –

Table 5 – continued from previous page

|              |                                                                                                                                        |
|--------------|----------------------------------------------------------------------------------------------------------------------------------------|
| $M_{5,9}^4$  | $m$ -vector: (103, 7, 92, 94, 11, 1)                                                                                                   |
| Perms.:      | (3, 2, 0, 1), (1, 0, 3, 2);(0, 1, 2, 3), (3, 1, 0, 2);(2, 0, 1, 3), (0, 1, 2, 3);(1, 2, 0, 3), (0, 1, 3, 2);(2, 0, 1, 3), (0, 2, 3, 1) |
| $M_{5,10}^4$ | $m$ -vector: (103, 7, 92, 94, 11, 1)                                                                                                   |
| Perms.:      | (3, 2, 0, 1), (1, 0, 3, 2);(0, 2, 1, 3), (2, 1, 0, 3);(2, 0, 1, 3), (0, 1, 2, 3);(1, 3, 0, 2), (0, 1, 3, 2);(2, 0, 1, 3), (0, 2, 3, 1) |
| $M_{5,11}^4$ | $m$ -vector: (15, 68, 88, 83, 12, 1)                                                                                                   |
| Perms.:      | (0, 2, 1, 3), (0, 2, 3, 1);(2, 1, 0, 3), (3, 0, 2, 1);(3, 2, 0, 1), (0, 3, 2, 1);(1, 3, 0, 2), (0, 1, 3, 2);(3, 1, 0, 2), (1, 0, 3, 2) |
| $M_{5,12}^4$ | $m$ -vector: (15, 68, 88, 83, 12, 1)                                                                                                   |
| Perms.:      | (0, 2, 1, 3), (0, 2, 3, 1);(1, 2, 0, 3), (3, 0, 1, 2);(3, 2, 0, 1), (0, 3, 2, 1);(1, 3, 0, 2), (0, 1, 3, 2);(3, 1, 0, 2), (1, 0, 3, 2) |
| $M_{5,13}^4$ | $m$ -vector: (51, 78, 89, 96, 12, 1)                                                                                                   |
| Perms.:      | (1, 3, 0, 2), (3, 0, 2, 1);(2, 3, 0, 1), (1, 2, 0, 3);(0, 2, 3, 1), (2, 0, 1, 3);(2, 3, 0, 1), (0, 3, 1, 2);(2, 0, 3, 1), (3, 1, 0, 2) |
| $M_{5,14}^4$ | $m$ -vector: (93, 30, 65, 18, 13, 1)                                                                                                   |
| Perms.:      | (3, 1, 0, 2), (0, 3, 2, 1);(1, 3, 0, 2), (3, 0, 1, 2);(1, 3, 0, 2), (2, 0, 3, 1);(0, 3, 1, 2), (3, 0, 1, 2);(1, 3, 0, 2), (2, 3, 0, 1) |
| $M_{5,15}^4$ | $m$ -vector: (44, 68, 38, 69, 13, 1)                                                                                                   |
| Perms.:      | (1, 0, 2, 3), (3, 0, 2, 1);(0, 1, 2, 3), (1, 0, 2, 3);(1, 2, 0, 3), (0, 2, 3, 1);(1, 3, 0, 2), (3, 2, 0, 1);(1, 0, 3, 2), (0, 3, 2, 1) |
| $M_{5,16}^4$ | $m$ -vector: (44, 68, 38, 69, 13, 1)                                                                                                   |
| Perms.:      | (1, 0, 2, 3), (3, 0, 2, 1);(0, 1, 2, 3), (1, 0, 2, 3);(1, 2, 0, 3), (0, 2, 3, 1);(2, 3, 0, 1), (3, 1, 0, 2);(1, 0, 3, 2), (0, 3, 2, 1) |
| $M_{5,17}^4$ | $m$ -vector: (59, 80, 16, 43, 14, 1)                                                                                                   |
| Perms.:      | (1, 3, 0, 2), (0, 3, 1, 2);(3, 0, 1, 2), (0, 3, 2, 1);(3, 0, 1, 2), (0, 3, 2, 1);(1, 3, 0, 2), (0, 3, 1, 2);(1, 3, 0, 2), (1, 0, 2, 3) |
| $M_{5,18}^4$ | $m$ -vector: (87, 40, 101, 100, 14, 1)                                                                                                 |
| Perms.:      | (3, 0, 1, 2), (1, 0, 3, 2);(0, 1, 2, 3), (0, 3, 1, 2);(3, 1, 0, 2), (0, 2, 3, 1);(2, 0, 3, 1), (3, 1, 0, 2);(3, 0, 2, 1), (2, 1, 0, 3) |
| $M_{5,19}^4$ | $m$ -vector: (68, 22, 19, 85, 15, 1)                                                                                                   |
| Perms.:      | (1, 2, 0, 3), (1, 3, 0, 2);(0, 1, 2, 3), (2, 0, 3, 1);(0, 1, 3, 2), (3, 0, 1, 2);(0, 2, 3, 1), (2, 0, 1, 3);(3, 2, 0, 1), (0, 2, 1, 3) |
| $M_{5,20}^4$ | $m$ -vector: (95, 93, 34, 39, 19, 1)                                                                                                   |
| Perms.:      | (0, 3, 1, 2), (2, 0, 1, 3);(0, 2, 3, 1), (0, 1, 2, 3);(2, 3, 0, 1), (3, 0, 2, 1);(1, 2, 0, 3), (2, 1, 0, 3);(3, 0, 2, 1), (0, 2, 3, 1) |
| $M_{5,21}^4$ | $m$ -vector: (95, 93, 34, 39, 19, 1)                                                                                                   |
| Perms.:      | (0, 3, 1, 2), (2, 0, 1, 3);(0, 2, 3, 1), (0, 1, 2, 3);(2, 3, 0, 1), (3, 0, 2, 1);(3, 2, 0, 1), (2, 1, 0, 3);(3, 0, 2, 1), (0, 2, 3, 1) |
| $M_{5,22}^4$ | $m$ -vector: (6, 68, 88, 93, 19, 1)                                                                                                    |
| Perms.:      | (1, 2, 0, 3), (2, 0, 1, 3);(2, 3, 0, 1), (0, 2, 1, 3);(1, 2, 0, 3), (3, 2, 0, 1);(0, 3, 2, 1), (0, 1, 2, 3);(3, 1, 0, 2), (1, 0, 3, 2) |
| $M_{5,23}^4$ | $m$ -vector: (25, 31, 68, 80, 23, 1)                                                                                                   |
| Perms.:      | (2, 0, 1, 3), (1, 2, 0, 3);(3, 0, 2, 1), (2, 1, 0, 3);(2, 0, 3, 1), (0, 2, 1, 3);(1, 3, 0, 2), (0, 3, 2, 1);(1, 3, 0, 2), (1, 0, 3, 2) |
| $M_{5,24}^4$ | $m$ -vector: (25, 31, 68, 80, 23, 1)                                                                                                   |
| Perms.:      | (2, 0, 1, 3), (1, 2, 0, 3);(3, 0, 2, 1), (2, 1, 0, 3);(2, 0, 3, 1), (0, 2, 1, 3);(1, 3, 0, 2), (0, 3, 1, 2);(1, 3, 0, 2), (1, 0, 3, 2) |
| $M_{5,25}^4$ | $m$ -vector: (17, 21, 79, 9, 24, 1)                                                                                                    |
| Perms.:      | (3, 0, 2, 1), (0, 3, 2, 1);(3, 0, 1, 2), (2, 3, 0, 1);(3, 0, 2, 1), (3, 0, 2, 1);(0, 3, 1, 2), (2, 3, 0, 1);(0, 1, 2, 3), (0, 2, 1, 3) |
| $M_{5,26}^4$ | $m$ -vector: (47, 14, 64, 29, 25, 1)                                                                                                   |
| Perms.:      | (1, 2, 0, 3), (1, 3, 0, 2);(0, 2, 3, 1), (0, 2, 1, 3);(1, 3, 0, 2), (3, 1, 0, 2);(1, 0, 3, 2), (2, 3, 0, 1);(3, 0, 2, 1), (2, 0, 1, 3) |
| $M_{5,27}^4$ | $m$ -vector: (52, 41, 20, 32, 25, 1)                                                                                                   |
| Perms.:      | (0, 3, 2, 1), (1, 0, 3, 2);(3, 2, 0, 1), (2, 1, 0, 3);(0, 1, 3, 2), (1, 3, 0, 2);(0, 3, 2, 1), (0, 2, 3, 1);(1, 3, 0, 2), (1, 0, 2, 3) |
| $M_{5,28}^4$ | $m$ -vector: (52, 16, 84, 103, 30, 1)                                                                                                  |
| Perms.:      | (0, 1, 3, 2), (3, 0, 2, 1);(0, 2, 1, 3), (3, 0, 2, 1);(2, 3, 0, 1), (0, 2, 1, 3);(2, 0, 1, 3), (2, 0, 3, 1);(0, 3, 2, 1), (1, 3, 0, 2) |
| $M_{5,29}^4$ | $m$ -vector: (83, 99, 65, 25, 32, 1)                                                                                                   |

continued on next page –

Table 5 – continued from previous page

|              |                                                                                                                                        |
|--------------|----------------------------------------------------------------------------------------------------------------------------------------|
| Perms.:      | (2, 0, 1, 3), (0, 2, 1, 3);(1, 2, 0, 3), (2, 0, 3, 1);(0, 3, 2, 1), (0, 2, 1, 3);(2, 0, 1, 3), (0, 2, 3, 1);(1, 0, 3, 2), (0, 2, 3, 1) |
| $M_{5,30}^4$ | $m$ -vector: (67, 26, 76, 58, 32, 1)                                                                                                   |
| Perms.:      | (1, 0, 3, 2), (1, 3, 0, 2);(0, 1, 3, 2), (3, 2, 0, 1);(0, 2, 3, 1), (3, 2, 0, 1);(0, 2, 1, 3), (0, 2, 3, 1);(1, 0, 2, 3), (1, 2, 0, 3) |
| $M_{5,31}^4$ | $m$ -vector: (17, 89, 21, 83, 33, 1)                                                                                                   |
| Perms.:      | (2, 1, 0, 3), (0, 3, 2, 1);(3, 2, 0, 1), (1, 2, 0, 3);(0, 3, 1, 2), (2, 0, 1, 3);(1, 2, 0, 3), (0, 1, 2, 3);(2, 0, 1, 3), (3, 0, 2, 1) |
| $M_{5,32}^4$ | $m$ -vector: (18, 78, 32, 22, 34, 1)                                                                                                   |
| Perms.:      | (3, 1, 0, 2), (1, 0, 3, 2);(0, 2, 1, 3), (3, 0, 1, 2);(2, 3, 0, 1), (3, 0, 2, 1);(0, 3, 1, 2), (2, 3, 0, 1);(3, 0, 1, 2), (0, 2, 3, 1) |
| $M_{5,33}^4$ | $m$ -vector: (25, 93, 40, 33, 39, 1)                                                                                                   |
| Perms.:      | (2, 0, 3, 1), (3, 0, 1, 2);(2, 1, 0, 3), (0, 2, 3, 1);(1, 2, 0, 3), (1, 0, 3, 2);(2, 1, 0, 3), (3, 2, 0, 1);(3, 0, 1, 2), (2, 0, 3, 1) |
| $M_{5,34}^4$ | $m$ -vector: (10, 103, 42, 68, 39, 1)                                                                                                  |
| Perms.:      | (1, 3, 0, 2), (1, 3, 0, 2);(1, 0, 3, 2), (2, 1, 0, 3);(2, 0, 3, 1), (1, 2, 0, 3);(0, 1, 2, 3), (2, 3, 0, 1);(0, 2, 3, 1), (3, 0, 1, 2) |
| $M_{5,35}^4$ | $m$ -vector: (84, 69, 65, 68, 39, 1)                                                                                                   |
| Perms.:      | (2, 3, 0, 1), (2, 0, 1, 3);(0, 1, 2, 3), (0, 2, 3, 1);(2, 1, 0, 3), (0, 1, 2, 3);(1, 0, 2, 3), (0, 3, 1, 2);(3, 2, 0, 1), (0, 2, 3, 1) |
| $M_{5,36}^4$ | $m$ -vector: (103, 75, 65, 96, 40, 1)                                                                                                  |
| Perms.:      | (1, 3, 0, 2), (1, 2, 0, 3);(3, 0, 2, 1), (1, 3, 0, 2);(1, 0, 2, 3), (2, 1, 0, 3);(0, 3, 2, 1), (0, 2, 3, 1);(3, 0, 2, 1), (0, 2, 3, 1) |
| $M_{5,37}^4$ | $m$ -vector: (48, 90, 22, 8, 41, 1)                                                                                                    |
| Perms.:      | (1, 3, 0, 2), (3, 1, 0, 2);(1, 0, 2, 3), (1, 0, 2, 3);(0, 1, 3, 2), (0, 3, 2, 1);(3, 0, 1, 2), (0, 3, 2, 1);(2, 1, 0, 3), (1, 3, 0, 2) |
| $M_{5,38}^4$ | $m$ -vector: (25, 6, 66, 78, 41, 1)                                                                                                    |
| Perms.:      | (0, 1, 2, 3), (1, 0, 2, 3);(0, 1, 3, 2), (1, 3, 0, 2);(1, 0, 3, 2), (0, 1, 2, 3);(2, 1, 0, 3), (3, 0, 1, 2);(2, 3, 0, 1), (2, 3, 0, 1) |
| $M_{5,39}^4$ | $m$ -vector: (97, 5, 45, 80, 42, 1)                                                                                                    |
| Perms.:      | (1, 0, 3, 2), (0, 1, 3, 2);(1, 3, 0, 2), (0, 3, 2, 1);(1, 0, 3, 2), (3, 1, 0, 2);(2, 0, 3, 1), (3, 0, 2, 1);(0, 1, 3, 2), (2, 3, 0, 1) |
| $M_{5,40}^4$ | $m$ -vector: (50, 58, 93, 83, 43, 1)                                                                                                   |
| Perms.:      | (3, 0, 2, 1), (3, 1, 0, 2);(0, 2, 3, 1), (0, 3, 2, 1);(3, 1, 0, 2), (3, 0, 2, 1);(3, 2, 0, 1), (3, 0, 2, 1);(3, 2, 0, 1), (1, 0, 3, 2) |
| $M_{5,41}^4$ | $m$ -vector: (60, 26, 24, 84, 44, 1)                                                                                                   |
| Perms.:      | (1, 0, 2, 3), (3, 0, 2, 1);(2, 1, 0, 3), (1, 2, 0, 3);(2, 0, 3, 1), (1, 3, 0, 2);(3, 0, 2, 1), (0, 1, 3, 2);(1, 0, 2, 3), (0, 1, 3, 2) |
| $M_{5,42}^4$ | $m$ -vector: (83, 16, 10, 95, 46, 1)                                                                                                   |
| Perms.:      | (2, 3, 0, 1), (0, 2, 1, 3);(3, 2, 0, 1), (1, 0, 3, 2);(0, 1, 2, 3), (0, 2, 3, 1);(3, 2, 0, 1), (1, 2, 0, 3);(3, 0, 2, 1), (0, 2, 1, 3) |
| $M_{5,43}^4$ | $m$ -vector: (15, 51, 70, 97, 46, 1)                                                                                                   |
| Perms.:      | (0, 1, 3, 2), (1, 0, 3, 2);(0, 1, 3, 2), (3, 2, 0, 1);(0, 3, 2, 1), (0, 2, 3, 1);(1, 2, 0, 3), (3, 0, 2, 1);(3, 1, 0, 2), (0, 1, 3, 2) |
| $M_{5,44}^4$ | $m$ -vector: (51, 52, 88, 6, 48, 1)                                                                                                    |
| Perms.:      | (1, 3, 0, 2), (0, 2, 3, 1);(1, 0, 2, 3), (2, 3, 0, 1);(3, 0, 1, 2), (3, 0, 2, 1);(3, 2, 0, 1), (0, 3, 2, 1);(2, 3, 0, 1), (1, 0, 3, 2) |
| $M_{5,45}^4$ | $m$ -vector: (51, 52, 88, 6, 48, 1)                                                                                                    |
| Perms.:      | (1, 3, 0, 2), (0, 2, 3, 1);(1, 0, 3, 2), (1, 3, 0, 2);(3, 0, 1, 2), (3, 0, 2, 1);(2, 3, 0, 1), (0, 3, 2, 1);(2, 3, 0, 1), (1, 0, 3, 2) |
| $M_{5,46}^4$ | $m$ -vector: (51, 52, 88, 6, 48, 1)                                                                                                    |
| Perms.:      | (1, 2, 0, 3), (0, 2, 3, 1);(1, 0, 2, 3), (2, 3, 0, 1);(3, 0, 2, 1), (3, 0, 2, 1);(3, 2, 0, 1), (0, 2, 3, 1);(2, 3, 0, 1), (1, 0, 3, 2) |
| $M_{5,47}^4$ | $m$ -vector: (51, 52, 88, 6, 48, 1)                                                                                                    |
| Perms.:      | (1, 2, 0, 3), (0, 2, 3, 1);(1, 0, 3, 2), (1, 3, 0, 2);(3, 0, 2, 1), (3, 0, 2, 1);(2, 3, 0, 1), (0, 2, 3, 1);(2, 3, 0, 1), (1, 0, 3, 2) |
| $M_{5,48}^4$ | $m$ -vector: (21, 91, 49, 10, 48, 1)                                                                                                   |
| Perms.:      | (3, 0, 2, 1), (3, 1, 0, 2);(0, 3, 2, 1), (1, 2, 0, 3);(0, 1, 3, 2), (2, 3, 0, 1);(3, 0, 1, 2), (0, 1, 3, 2);(3, 0, 2, 1), (3, 0, 2, 1) |
| $M_{5,49}^4$ | $m$ -vector: (22, 103, 20, 90, 48, 1)                                                                                                  |
| Perms.:      | (3, 0, 2, 1), (0, 3, 2, 1);(3, 0, 2, 1), (3, 2, 0, 1);(3, 0, 2, 1), (1, 0, 2, 3);(0, 3, 1, 2), (1, 0, 2, 3);(2, 3, 0, 1), (0, 3, 2, 1) |

continued on next page –



Table 5 – continued from previous page

|              |                                                                                                                                        |
|--------------|----------------------------------------------------------------------------------------------------------------------------------------|
| $M_{5,50}^4$ | $m$ -vector: (22, 103, 20, 90, 48, 1)                                                                                                  |
| Perms.:      | (3, 0, 1, 2), (0, 3, 1, 2);(3, 0, 2, 1), (3, 2, 0, 1);(2, 0, 3, 1), (2, 0, 1, 3);(0, 3, 1, 2), (1, 0, 2, 3);(2, 3, 0, 1), (0, 3, 2, 1) |
| $M_{5,51}^4$ | $m$ -vector: (47, 26, 59, 49, 58, 1)                                                                                                   |
| Perms.:      | (2, 1, 0, 3), (1, 0, 2, 3);(0, 1, 2, 3), (3, 0, 2, 1);(0, 2, 1, 3), (2, 0, 1, 3);(1, 2, 0, 3), (3, 2, 0, 1);(3, 0, 1, 2), (1, 0, 3, 2) |
| $M_{5,52}^4$ | $m$ -vector: (97, 21, 70, 64, 59, 1)                                                                                                   |
| Perms.:      | (1, 2, 0, 3), (1, 2, 0, 3);(0, 2, 3, 1), (0, 1, 3, 2);(2, 3, 0, 1), (3, 0, 2, 1);(1, 3, 0, 2), (1, 3, 0, 2);(3, 0, 1, 2), (3, 0, 1, 2) |
| $M_{5,53}^4$ | $m$ -vector: (11, 52, 16, 88, 59, 1)                                                                                                   |
| Perms.:      | (2, 0, 3, 1), (2, 1, 0, 3);(3, 0, 1, 2), (1, 0, 2, 3);(3, 1, 0, 2), (1, 0, 3, 2);(3, 1, 0, 2), (3, 0, 1, 2);(2, 3, 0, 1), (0, 2, 1, 3) |
| $M_{5,54}^4$ | $m$ -vector: (60, 52, 16, 88, 59, 1)                                                                                                   |
| Perms.:      | (1, 0, 3, 2), (2, 1, 0, 3);(3, 0, 1, 2), (1, 0, 2, 3);(3, 2, 0, 1), (2, 0, 3, 1);(3, 1, 0, 2), (3, 0, 1, 2);(2, 3, 0, 1), (3, 0, 1, 2) |
| $M_{5,55}^4$ | $m$ -vector: (57, 61, 41, 103, 60, 1)                                                                                                  |
| Perms.:      | (1, 3, 0, 2), (0, 2, 3, 1);(3, 1, 0, 2), (1, 3, 0, 2);(0, 1, 3, 2), (3, 0, 1, 2);(3, 1, 0, 2), (0, 1, 3, 2);(1, 0, 2, 3), (2, 1, 0, 3) |
| $M_{5,56}^4$ | $m$ -vector: (94, 101, 63, 68, 65, 1)                                                                                                  |
| Perms.:      | (0, 3, 2, 1), (0, 2, 1, 3);(1, 3, 0, 2), (1, 0, 2, 3);(0, 1, 2, 3), (0, 3, 1, 2);(1, 0, 2, 3), (0, 2, 3, 1);(2, 0, 3, 1), (2, 1, 0, 3) |
| $M_{5,57}^4$ | $m$ -vector: (39, 77, 12, 5, 68, 1)                                                                                                    |
| Perms.:      | (1, 2, 0, 3), (0, 3, 1, 2);(1, 3, 0, 2), (3, 1, 0, 2);(1, 0, 3, 2), (0, 1, 2, 3);(1, 2, 0, 3), (3, 0, 2, 1);(3, 2, 0, 1), (3, 0, 2, 1) |
| $M_{5,58}^4$ | $m$ -vector: (24, 39, 69, 43, 68, 1)                                                                                                   |
| Perms.:      | (3, 0, 1, 2), (3, 1, 0, 2);(0, 3, 2, 1), (1, 0, 2, 3);(0, 3, 1, 2), (1, 0, 2, 3);(2, 3, 0, 1), (3, 0, 1, 2);(3, 1, 0, 2), (1, 0, 3, 2) |
| $M_{5,59}^4$ | $m$ -vector: (24, 39, 69, 43, 68, 1)                                                                                                   |
| Perms.:      | (3, 0, 1, 2), (3, 1, 0, 2);(0, 3, 1, 2), (1, 0, 2, 3);(0, 3, 1, 2), (1, 0, 2, 3);(2, 3, 0, 1), (3, 0, 1, 2);(3, 1, 0, 2), (1, 0, 3, 2) |
| $M_{5,60}^4$ | $m$ -vector: (70, 24, 44, 99, 68, 1)                                                                                                   |
| Perms.:      | (1, 0, 2, 3), (1, 0, 2, 3);(0, 1, 2, 3), (0, 2, 3, 1);(3, 0, 2, 1), (0, 3, 1, 2);(1, 0, 2, 3), (1, 0, 3, 2);(3, 1, 0, 2), (3, 1, 0, 2) |
| $M_{5,61}^4$ | $m$ -vector: (33, 83, 67, 7, 69, 1)                                                                                                    |
| Perms.:      | (1, 3, 0, 2), (0, 1, 3, 2);(2, 0, 1, 3), (0, 1, 3, 2);(1, 0, 2, 3), (3, 0, 2, 1);(3, 2, 0, 1), (1, 0, 3, 2);(0, 3, 2, 1), (1, 2, 0, 3) |
| $M_{5,62}^4$ | $m$ -vector: (100, 43, 94, 8, 69, 1)                                                                                                   |
| Perms.:      | (3, 1, 0, 2), (3, 0, 1, 2);(0, 1, 2, 3), (2, 0, 3, 1);(0, 3, 2, 1), (2, 0, 1, 3);(0, 1, 2, 3), (2, 3, 0, 1);(0, 1, 3, 2), (0, 2, 1, 3) |
| $M_{5,63}^4$ | $m$ -vector: (100, 43, 94, 8, 69, 1)                                                                                                   |
| Perms.:      | (3, 2, 0, 1), (3, 0, 2, 1);(0, 1, 2, 3), (2, 0, 3, 1);(0, 2, 3, 1), (2, 1, 0, 3);(0, 1, 2, 3), (2, 3, 0, 1);(1, 0, 3, 2), (0, 3, 1, 2) |
| $M_{5,64}^4$ | $m$ -vector: (39, 85, 41, 33, 69, 1)                                                                                                   |
| Perms.:      | (3, 0, 1, 2), (0, 3, 2, 1);(3, 0, 2, 1), (2, 0, 1, 3);(3, 1, 0, 2), (0, 3, 2, 1);(1, 2, 0, 3), (0, 3, 2, 1);(3, 2, 0, 1), (0, 2, 3, 1) |
| $M_{5,65}^4$ | $m$ -vector: (52, 20, 68, 42, 77, 1)                                                                                                   |
| Perms.:      | (0, 3, 1, 2), (2, 1, 0, 3);(1, 0, 2, 3), (1, 2, 0, 3);(0, 3, 2, 1), (3, 0, 1, 2);(0, 3, 2, 1), (1, 0, 2, 3);(0, 1, 3, 2), (3, 2, 0, 1) |
| $M_{5,66}^4$ | $m$ -vector: (31, 95, 85, 86, 80, 1)                                                                                                   |
| Perms.:      | (3, 1, 0, 2), (2, 1, 0, 3);(0, 3, 2, 1), (2, 3, 0, 1);(3, 0, 1, 2), (0, 3, 2, 1);(3, 1, 0, 2), (2, 0, 3, 1);(0, 2, 3, 1), (0, 2, 1, 3) |
| $M_{5,67}^4$ | $m$ -vector: (87, 23, 57, 77, 84, 1)                                                                                                   |
| Perms.:      | (2, 0, 3, 1), (0, 3, 2, 1);(2, 1, 0, 3), (2, 3, 0, 1);(3, 0, 1, 2), (0, 3, 1, 2);(3, 0, 2, 1), (0, 2, 1, 3);(1, 0, 3, 2), (1, 0, 3, 2) |
| $M_{5,68}^4$ | $m$ -vector: (31, 64, 25, 41, 87, 1)                                                                                                   |
| Perms.:      | (1, 0, 2, 3), (0, 1, 3, 2);(2, 3, 0, 1), (3, 0, 1, 2);(0, 1, 3, 2), (3, 2, 0, 1);(2, 0, 3, 1), (0, 3, 1, 2);(3, 2, 0, 1), (3, 0, 2, 1) |
| $M_{5,69}^4$ | $m$ -vector: (38, 8, 44, 13, 89, 1)                                                                                                    |
| Perms.:      | (3, 0, 1, 2), (0, 1, 3, 2);(2, 3, 0, 1), (1, 0, 3, 2);(3, 2, 0, 1), (2, 3, 0, 1);(1, 0, 3, 2), (1, 2, 0, 3);(0, 1, 2, 3), (3, 0, 2, 1) |
| $M_{5,70}^4$ | $m$ -vector: (38, 8, 44, 13, 89, 1)                                                                                                    |

continued on next page –

Table 5 – continued from previous page

|              |                                                                                                                                        |
|--------------|----------------------------------------------------------------------------------------------------------------------------------------|
| Perms.:      | (3, 0, 1, 2), (0, 1, 3, 2);(2, 3, 0, 1), (1, 0, 3, 2);(3, 2, 0, 1), (2, 3, 0, 1);(1, 0, 3, 2), (1, 2, 0, 3);(0, 1, 2, 3), (3, 0, 1, 2) |
| $M_{5,71}^4$ | $m$ -vector: (38, 8, 44, 13, 89, 1)                                                                                                    |
| Perms.:      | (3, 0, 1, 2), (0, 1, 3, 2);(2, 3, 0, 1), (1, 0, 3, 2);(3, 2, 0, 1), (2, 3, 0, 1);(1, 0, 3, 2), (1, 2, 0, 3);(0, 3, 2, 1), (3, 0, 2, 1) |
| $M_{5,72}^4$ | $m$ -vector: (38, 8, 44, 13, 89, 1)                                                                                                    |
| Perms.:      | (3, 0, 1, 2), (0, 1, 3, 2);(2, 3, 0, 1), (1, 0, 3, 2);(3, 2, 0, 1), (2, 3, 0, 1);(1, 0, 3, 2), (1, 2, 0, 3);(0, 3, 2, 1), (3, 0, 1, 2) |

Table 6: 5-dimensional handlebodies with  $k = 2$ 

|             |                                                                                                                                                                                                                                                                                                                                                                                                                                                                 |
|-------------|-----------------------------------------------------------------------------------------------------------------------------------------------------------------------------------------------------------------------------------------------------------------------------------------------------------------------------------------------------------------------------------------------------------------------------------------------------------------|
| $M_{2,1}^5$ | $m$ -vector: (44, 8, 1)                                                                                                                                                                                                                                                                                                                                                                                                                                         |
| Perms.:     | $\sigma_2 = (0, 3, 1, 4, 2)$ , $\tau_2 = (0, 4, 3, 2, 1)$ ;<br>$\sigma_1 = (1, 2, 0, 3, 4)$ , $\tau_1 = (0, 2, 4, 1, 3)$                                                                                                                                                                                                                                                                                                                                        |
| Treotypes:  | $\Delta(\sigma_2, \tau_2) = \{(2, 2), (2, 3), (2, 4), (3, 2), (4, 2), (4, 3), (4, 4), (4, 5), (5, 2), (5, 3)\}$ ,<br>$\Delta(\sigma_1, \tau_1) = \{(1, 3), (2, 3), (2, 5), (4, 2), (4, 3), (4, 5), (5, 2), (5, 3), (5, 4), (5, 5)\}$                                                                                                                                                                                                                            |
| Orb. reps.: | $\langle 0, 1, 2, 3, 4, 5 \rangle$ , $\langle 0, 1, 2, 3, 14, 69 \rangle$ , $\langle 0, 1, 12, 20, 67, 69 \rangle$ , $\langle 0, 2, 4, 16, 24, 32 \rangle$ , $\langle 0, 4, 16, 24, 32, 40 \rangle$ ,<br>$\langle 0, 7, 16, 32, 40, 61 \rangle$ , $\langle 0, 7, 17, 32, 40, 61 \rangle$ , $\langle 0, 6, 27, 37, 44, 54 \rangle$ , $\langle 0, 7, 17, 34, 44, 61 \rangle$ , $\langle 0, 8, 16, 24, 32, 40 \rangle$ ,<br>$\langle 0, 8, 16, 32, 40, 61 \rangle$ |
| $M_{2,2}^5$ | $m$ -vector: (44, 8, 1)                                                                                                                                                                                                                                                                                                                                                                                                                                         |
| Perms.:     | $\sigma_2 = (0, 3, 1, 4, 2)$ , $\tau_2 = (0, 4, 3, 2, 1)$ ;<br>$\sigma_1 = (2, 1, 0, 3, 4)$ , $\tau_1 = (0, 3, 4, 1, 2)$                                                                                                                                                                                                                                                                                                                                        |
| Treotypes:  | $\Delta(\sigma_2, \tau_2) = \{(2, 2), (2, 3), (2, 4), (3, 2), (4, 2), (4, 3), (4, 4), (4, 5), (5, 2), (5, 3)\}$ ,<br>$\Delta(\sigma_1, \tau_1) = \{(1, 2), (1, 3), (2, 3), (4, 2), (4, 3), (4, 5), (5, 2), (5, 3), (5, 4), (5, 5)\}$                                                                                                                                                                                                                            |
| Orb. reps.: | $\langle 0, 1, 2, 3, 4, 5 \rangle$ , $\langle 0, 1, 2, 3, 14, 69 \rangle$ , $\langle 0, 1, 12, 20, 67, 69 \rangle$ , $\langle 0, 2, 4, 16, 24, 32 \rangle$ , $\langle 0, 4, 16, 24, 32, 40 \rangle$ ,<br>$\langle 0, 7, 17, 32, 40, 61 \rangle$ , $\langle 0, 6, 27, 37, 44, 54 \rangle$ , $\langle 0, 7, 17, 34, 44, 61 \rangle$ , $\langle 0, 8, 16, 24, 32, 40 \rangle$ , $\langle 0, 8, 16, 32, 40, 61 \rangle$ ,<br>$\langle 0, 8, 17, 32, 40, 61 \rangle$ |

Table 7: 5-dimensional handlebodies with  $k = 3$ 

|             |                                                                                                                                                                                                                                                                                                                                                                                                                                                                                                                                                                                                                                                                                        |
|-------------|----------------------------------------------------------------------------------------------------------------------------------------------------------------------------------------------------------------------------------------------------------------------------------------------------------------------------------------------------------------------------------------------------------------------------------------------------------------------------------------------------------------------------------------------------------------------------------------------------------------------------------------------------------------------------------------|
| $M_{3,1}^5$ | $m$ -vector: (62, 43, 12, 1)                                                                                                                                                                                                                                                                                                                                                                                                                                                                                                                                                                                                                                                           |
| Perms.:     | $\sigma_3 = (0, 3, 2, 4, 1)$ , $\tau_3 = (3, 4, 2, 0, 1)$ ;<br>$\sigma_2 = (3, 0, 2, 1, 4)$ , $\tau_2 = (2, 4, 0, 3, 1)$ ;<br>$\sigma_1 = (0, 1, 2, 3, 4)$ , $\tau_1 = (1, 0, 3, 4, 2)$                                                                                                                                                                                                                                                                                                                                                                                                                                                                                                |
| Treotypes:  | $\Delta(\sigma_3, \tau_3) = \{(2, 1), (2, 2), (2, 3), (3, 1), (3, 2), (4, 1), (4, 2), (4, 3), (4, 5), (5, 2)\}$ ,<br>$\Delta(\sigma_2, \tau_2) = \{(1, 1), (1, 2), (1, 4), (3, 2), (3, 4), (4, 2), (5, 1), (5, 2), (5, 4), (5, 5)\}$ ,<br>$\Delta(\sigma_1, \tau_1) = \{(2, 4), (3, 3), (3, 4), (4, 3), (4, 4), (4, 5), (5, 1), (5, 3), (5, 4), (5, 5)\}$                                                                                                                                                                                                                                                                                                                              |
| Orb. reps.: | $\langle 0, 1, 2, 3, 4, 5 \rangle$ , $\langle 0, 1, 2, 3, 22, 99 \rangle$ , $\langle 0, 1, 2, 10, 22, 99 \rangle$ , $\langle 0, 2, 4, 12, 24, 36 \rangle$ ,<br>$\langle 0, 4, 12, 24, 36, 60 \rangle$ , $\langle 0, 6, 39, 55, 78, 94 \rangle$ , $\langle 0, 6, 39, 64, 78, 94 \rangle$ , $\langle 0, 7, 23, 46, 62, 85 \rangle$ ,<br>$\langle 0, 12, 24, 36, 48, 60 \rangle$ , $\langle 0, 12, 24, 50, 65, 77 \rangle$ , $\langle 0, 11, 26, 41, 53, 77 \rangle$ , $\langle 0, 11, 26, 41, 53, 84 \rangle$ ,<br>$\langle 0, 13, 28, 43, 71, 86 \rangle$ , $\langle 0, 13, 28, 46, 71, 85 \rangle$ , $\langle 0, 13, 28, 46, 71, 86 \rangle$ , $\langle 0, 11, 26, 41, 54, 84 \rangle$ |
| $M_{3,2}^5$ | $m$ -vector: (65, 6, 84, 1)                                                                                                                                                                                                                                                                                                                                                                                                                                                                                                                                                                                                                                                            |
| Perms.:     | $\sigma_3 = (3, 2, 1, 0, 4)$ , $\tau_3 = (0, 1, 2, 3, 4)$ ;<br>$\sigma_2 = (2, 0, 4, 3, 1)$ , $\tau_2 = (3, 2, 0, 4, 1)$ ;<br>$\sigma_1 = (1, 4, 3, 0, 2)$ , $\tau_1 = (4, 0, 3, 2, 1)$                                                                                                                                                                                                                                                                                                                                                                                                                                                                                                |
| Treotypes:  | $\Delta(\sigma_3, \tau_3) = \{(1, 3), (1, 4), (1, 5), (2, 4), (2, 5), (3, 5), (5, 2), (5, 3), (5, 4), (5, 5)\}$ ,<br>$\Delta(\sigma_2, \tau_2) = \{(1, 1), (1, 4), (3, 1), (3, 2), (3, 4), (3, 5), (4, 1), (4, 2), (4, 4), (5, 4)\}$ ,<br>$\Delta(\sigma_1, \tau_1) = \{(1, 1), (2, 1), (2, 3), (2, 4), (2, 5), (3, 1), (3, 3), (3, 4), (5, 1), (5, 3)\}$                                                                                                                                                                                                                                                                                                                              |
| Orb. reps.: | $\langle 0, 1, 2, 3, 4, 5 \rangle$ , $\langle 0, 1, 2, 3, 5, 16 \rangle$ , $\langle 0, 1, 2, 5, 16, 33 \rangle$ , $\langle 0, 1, 5, 16, 33, 50 \rangle$ ,<br>$\langle 0, 5, 16, 33, 50, 67 \rangle$ , $\langle 0, 6, 12, 18, 24, 30 \rangle$ , $\langle 0, 6, 12, 18, 30, 65 \rangle$ , $\langle 0, 6, 12, 24, 30, 50 \rangle$ ,<br>$\langle 0, 6, 12, 24, 33, 50 \rangle$ , $\langle 0, 6, 24, 33, 50, 84 \rangle$ , $\langle 0, 6, 18, 53, 82, 89 \rangle$ , $\langle 0, 6, 46, 53, 82, 89 \rangle$ ,<br>$\langle 0, 7, 19, 29, 65, 72 \rangle$ , $\langle 0, 8, 17, 34, 68, 85 \rangle$ , $\langle 0, 16, 33, 50, 67, 84 \rangle$ , $\langle 0, 7, 29, 36, 65, 72 \rangle$          |

Table 8: 6-dimensional handlebodies with  $k = 1$ 

|              |                                                                                                                                                                                                                                                                                                                               |
|--------------|-------------------------------------------------------------------------------------------------------------------------------------------------------------------------------------------------------------------------------------------------------------------------------------------------------------------------------|
| $M_{1,65}^6$ | $m$ -vector: (16, 1)                                                                                                                                                                                                                                                                                                          |
| Perms.:      | $\sigma_1 = (3, 0, 4, 5, 1, 2), \quad \tau_1 = (1, 2, 4, 0, 5, 3)$                                                                                                                                                                                                                                                            |
| Treotypes:   | $\Delta(\sigma_1, \tau_1) = \{(1, 3), (1, 5), (1, 6), (3, 2), (3, 3), (3, 5), (3, 6),$<br>$(4, 1), (4, 2), (4, 3), (4, 5), (4, 6), (5, 5), (6, 3), (6, 5)\}$                                                                                                                                                                  |
| Orb. reps.:  | $\langle 0, 1, 2, 3, 4, 5, 6 \rangle, \quad \langle 0, 1, 2, 3, 22, 52, 53 \rangle, \quad \langle 0, 1, 3, 4, 6, 25, 48 \rangle, \quad \langle 0, 1, 3, 4, 25, 41, 48 \rangle,$<br>$\langle 0, 1, 22, 29, 38, 45, 52 \rangle, \quad \langle 0, 4, 16, 25, 32, 41, 48 \rangle, \quad \langle 0, 7, 14, 23, 30, 39, 46 \rangle$ |
| $M_{1,66}^6$ | $m$ -vector: (16, 1)                                                                                                                                                                                                                                                                                                          |
| Perms.:      | $\sigma_1 = (3, 0, 4, 5, 1, 2), \quad \tau_1 = (1, 3, 4, 0, 2, 5)$                                                                                                                                                                                                                                                            |
| Treotypes:   | $\Delta(\sigma_1, \tau_1) = \{(1, 2), (1, 3), (1, 6), (3, 2), (3, 3), (3, 5), (3, 6),$<br>$(4, 1), (4, 2), (4, 3), (4, 5), (4, 6), (5, 6), (6, 3), (6, 6)\}$                                                                                                                                                                  |
| Orb. reps.:  | $\langle 0, 1, 2, 3, 4, 5, 6 \rangle, \quad \langle 0, 1, 2, 3, 38, 52, 53 \rangle, \quad \langle 0, 1, 3, 4, 6, 41, 48 \rangle, \quad \langle 0, 1, 3, 4, 32, 41, 48 \rangle,$<br>$\langle 0, 1, 22, 29, 38, 45, 52 \rangle, \quad \langle 0, 4, 16, 25, 32, 41, 48 \rangle, \quad \langle 0, 7, 14, 23, 30, 39, 46 \rangle$ |
| $M_{1,67}^6$ | $m$ -vector: (16, 1)                                                                                                                                                                                                                                                                                                          |
| Perms.:      | $(3, 0, 4, 5, 1, 2), (1, 2, 4, 0, 3, 5)$                                                                                                                                                                                                                                                                                      |
| $M_{1,68}^6$ | $m$ -vector: (16, 1)                                                                                                                                                                                                                                                                                                          |
| Perms.:      | $(3, 0, 5, 4, 2, 1), (1, 2, 4, 0, 5, 3)$                                                                                                                                                                                                                                                                                      |
| $M_{1,69}^6$ | $m$ -vector: (16, 1)                                                                                                                                                                                                                                                                                                          |
| Perms.:      | $(3, 0, 5, 4, 2, 1), (1, 3, 4, 0, 2, 5)$                                                                                                                                                                                                                                                                                      |
| $M_{1,70}^6$ | $m$ -vector: (16, 1)                                                                                                                                                                                                                                                                                                          |
| Perms.:      | $(3, 0, 5, 4, 2, 1), (1, 2, 4, 0, 3, 5)$                                                                                                                                                                                                                                                                                      |
| $M_{1,71}^6$ | $m$ -vector: (24, 1)                                                                                                                                                                                                                                                                                                          |
| Perms.:      | $(4, 2, 0, 5, 3, 1), (1, 4, 2, 3, 0, 5)$                                                                                                                                                                                                                                                                                      |
| $M_{1,72}^6$ | $m$ -vector: (24, 1)                                                                                                                                                                                                                                                                                                          |
| Perms.:      | $(4, 2, 0, 1, 3, 5), (1, 4, 2, 3, 0, 5)$                                                                                                                                                                                                                                                                                      |
| $M_{1,73}^6$ | $m$ -vector: (24, 1)                                                                                                                                                                                                                                                                                                          |
| Perms.:      | $(2, 4, 0, 5, 3, 1), (1, 4, 2, 3, 0, 5)$                                                                                                                                                                                                                                                                                      |
| $M_{1,74}^6$ | $m$ -vector: (24, 1)                                                                                                                                                                                                                                                                                                          |
| Perms.:      | $(2, 4, 0, 1, 3, 5), (1, 4, 2, 3, 0, 5)$                                                                                                                                                                                                                                                                                      |
| $M_{1,75}^6$ | $m$ -vector: (24, 1)                                                                                                                                                                                                                                                                                                          |
| Perms.:      | $(5, 1, 0, 2, 3, 4), (0, 3, 2, 4, 1, 5)$                                                                                                                                                                                                                                                                                      |
| $M_{1,76}^6$ | $m$ -vector: (24, 1)                                                                                                                                                                                                                                                                                                          |
| Perms.:      | $(5, 1, 0, 2, 3, 4), (0, 2, 3, 4, 1, 5)$                                                                                                                                                                                                                                                                                      |
| $M_{1,77}^6$ | $m$ -vector: (24, 1)                                                                                                                                                                                                                                                                                                          |
| Perms.:      | $(5, 1, 0, 2, 3, 4), (2, 5, 1, 3, 0, 4)$                                                                                                                                                                                                                                                                                      |
| $M_{1,78}^6$ | $m$ -vector: (24, 1)                                                                                                                                                                                                                                                                                                          |
| Perms.:      | $(5, 1, 0, 2, 3, 4), (3, 5, 1, 2, 0, 4)$                                                                                                                                                                                                                                                                                      |
| $M_{1,79}^6$ | $m$ -vector: (24, 1)                                                                                                                                                                                                                                                                                                          |
| Perms.:      | $(5, 1, 0, 4, 3, 2), (0, 3, 2, 4, 1, 5)$                                                                                                                                                                                                                                                                                      |
| $M_{1,80}^6$ | $m$ -vector: (24, 1)                                                                                                                                                                                                                                                                                                          |
| Perms.:      | $(5, 1, 0, 4, 3, 2), (0, 2, 3, 4, 1, 5)$                                                                                                                                                                                                                                                                                      |
| $M_{1,81}^6$ | $m$ -vector: (24, 1)                                                                                                                                                                                                                                                                                                          |
| Perms.:      | $(5, 1, 0, 4, 3, 2), (2, 5, 1, 3, 0, 4)$                                                                                                                                                                                                                                                                                      |
| $M_{1,82}^6$ | $m$ -vector: (24, 1)                                                                                                                                                                                                                                                                                                          |

continued on next page –

Table 8 – continued from previous page

|              |                                        |
|--------------|----------------------------------------|
| Perms.:      | (5, 1, 0, 4, 3, 2), (3, 5, 1, 2, 0, 4) |
| $M_{1,83}^6$ | $m$ -vector: (24, 1)                   |
| Perms.:      | (1, 5, 0, 4, 3, 2), (0, 3, 2, 4, 1, 5) |
| $M_{1,84}^6$ | $m$ -vector: (24, 1)                   |
| Perms.:      | (1, 5, 0, 4, 3, 2), (0, 2, 3, 4, 1, 5) |
| $M_{1,85}^6$ | $m$ -vector: (24, 1)                   |
| Perms.:      | (1, 5, 0, 4, 3, 2), (2, 5, 1, 3, 0, 4) |
| $M_{1,86}^6$ | $m$ -vector: (24, 1)                   |
| Perms.:      | (1, 5, 0, 4, 3, 2), (3, 5, 1, 2, 0, 4) |
| $M_{1,87}^6$ | $m$ -vector: (24, 1)                   |
| Perms.:      | (1, 5, 0, 2, 3, 4), (0, 3, 2, 4, 1, 5) |
| $M_{1,88}^6$ | $m$ -vector: (24, 1)                   |
| Perms.:      | (1, 5, 0, 2, 3, 4), (0, 2, 3, 4, 1, 5) |
| $M_{1,89}^6$ | $m$ -vector: (24, 1)                   |
| Perms.:      | (1, 5, 0, 2, 3, 4), (2, 5, 1, 3, 0, 4) |
| $M_{1,90}^6$ | $m$ -vector: (24, 1)                   |
| Perms.:      | (1, 5, 0, 2, 3, 4), (3, 5, 1, 2, 0, 4) |

Table 9: 6-dimensional handlebodies with  $k = 2$ 

|             |                                                                                                                                                                                                                                                                                                                                                                                                                                                                                                                                                                                                                               |
|-------------|-------------------------------------------------------------------------------------------------------------------------------------------------------------------------------------------------------------------------------------------------------------------------------------------------------------------------------------------------------------------------------------------------------------------------------------------------------------------------------------------------------------------------------------------------------------------------------------------------------------------------------|
| $M_{2,1}^6$ | $m$ -vector: (87, 7, 1)                                                                                                                                                                                                                                                                                                                                                                                                                                                                                                                                                                                                       |
| Perms.:     | $\sigma_2 = (1, 4, 5, 0, 2, 3), \quad \tau_2 = (0, 5, 4, 3, 2, 1);$<br>$\sigma_1 = (2, 5, 4, 3, 0, 1), \quad \tau_1 = (5, 4, 2, 3, 0, 1)$                                                                                                                                                                                                                                                                                                                                                                                                                                                                                     |
| Treotypes:  | $\Delta(\sigma_2, \tau_2) = \{(1, 2), (2, 2), (2, 3), (2, 4), (2, 5), (3, 2), (3, 3),$<br>$(3, 4), (3, 5), (3, 6), (5, 2), (5, 3), (6, 2), (6, 3), (6, 4)\},$<br>$\Delta(\sigma_1, \tau_1) = \{(1, 1), (1, 2), (2, 1), (2, 2), (2, 3), (2, 4), (2, 6),$<br>$(3, 1), (3, 2), (3, 3), (3, 4), (4, 1), (4, 2), (4, 4), (6, 1)\}$                                                                                                                                                                                                                                                                                                 |
| Orb. reps.: | $\langle 0, 1, 2, 3, 4, 5, 6 \rangle, \quad \langle 0, 1, 2, 3, 5, 6, 14 \rangle, \quad \langle 0, 1, 3, 4, 12, 19, 95 \rangle, \quad \langle 0, 1, 4, 12, 19, 26, 95 \rangle,$<br>$\langle 0, 1, 12, 19, 26, 33, 95 \rangle, \quad \langle 0, 3, 14, 21, 28, 35, 42 \rangle, \quad \langle 0, 7, 14, 21, 28, 35, 42 \rangle, \quad \langle 0, 7, 14, 21, 28, 42, 87 \rangle,$<br>$\langle 0, 7, 14, 21, 28, 77, 87 \rangle, \quad \langle 0, 7, 14, 43, 63, 73, 83 \rangle, \quad \langle 0, 7, 43, 53, 63, 73, 83 \rangle, \quad \langle 0, 10, 20, 30, 40, 54, 77 \rangle,$<br>$\langle 0, 10, 20, 30, 40, 50, 60 \rangle$ |
| $M_{2,2}^6$ | $m$ -vector: (87, 7, 1)                                                                                                                                                                                                                                                                                                                                                                                                                                                                                                                                                                                                       |
| Perms.:     | $\sigma_2 = (1, 4, 5, 0, 2, 3), \quad \tau_2 = (0, 5, 3, 4, 2, 1);$<br>$\sigma_1 = (2, 4, 5, 3, 0, 1), \quad \tau_1 = (5, 4, 2, 3, 0, 1)$                                                                                                                                                                                                                                                                                                                                                                                                                                                                                     |
| Treotypes:  | $\Delta(\sigma_2, \tau_2) = \{(1, 2), (2, 2), (2, 3), (2, 4), (2, 5), (3, 2), (3, 3),$<br>$(3, 4), (3, 5), (3, 6), (5, 2), (5, 4), (6, 2), (6, 3), (6, 4)\},$<br>$\Delta(\sigma_1, \tau_1) = \{(1, 1), (1, 2), (2, 1), (2, 2), (2, 3), (2, 4), (3, 1),$<br>$(3, 2), (3, 3), (3, 4), (3, 6), (4, 1), (4, 2), (4, 4), (6, 1)\}$                                                                                                                                                                                                                                                                                                 |
| Orb. reps.: | $\langle 0, 1, 2, 3, 4, 5, 6 \rangle, \quad \langle 0, 1, 2, 3, 5, 6, 14 \rangle, \quad \langle 0, 1, 3, 4, 12, 26, 95 \rangle, \quad \langle 0, 1, 4, 12, 19, 26, 95 \rangle,$<br>$\langle 0, 1, 12, 19, 26, 33, 95 \rangle, \quad \langle 0, 3, 14, 21, 28, 35, 42 \rangle, \quad \langle 0, 7, 14, 21, 28, 35, 42 \rangle, \quad \langle 0, 7, 14, 21, 28, 42, 87 \rangle,$<br>$\langle 0, 7, 14, 21, 28, 77, 87 \rangle, \quad \langle 0, 7, 14, 43, 63, 73, 83 \rangle, \quad \langle 0, 7, 43, 53, 63, 73, 83 \rangle, \quad \langle 0, 10, 20, 30, 40, 61, 77 \rangle,$<br>$\langle 0, 10, 20, 30, 40, 50, 60 \rangle$ |
| $M_{2,3}^6$ | $m$ -vector: (88, 7, 1)                                                                                                                                                                                                                                                                                                                                                                                                                                                                                                                                                                                                       |
| Perms.:     | (2, 4, 1, 5, 0, 3), (0, 5, 4, 2, 3, 1); (3, 4, 5, 0, 1, 2), (4, 5, 3, 2, 0, 1)                                                                                                                                                                                                                                                                                                                                                                                                                                                                                                                                                |
| $M_{2,4}^6$ | $m$ -vector: (88, 7, 1)                                                                                                                                                                                                                                                                                                                                                                                                                                                                                                                                                                                                       |
| Perms.:     | (2, 4, 1, 5, 0, 3), (0, 5, 4, 2, 3, 1); (3, 4, 5, 0, 1, 2), (5, 4, 3, 2, 0, 1)                                                                                                                                                                                                                                                                                                                                                                                                                                                                                                                                                |
| $M_{2,5}^6$ | $m$ -vector: (88, 7, 1)                                                                                                                                                                                                                                                                                                                                                                                                                                                                                                                                                                                                       |
| Perms.:     | (2, 4, 1, 5, 0, 3), (0, 5, 4, 3, 2, 1); (3, 5, 4, 0, 1, 2), (4, 5, 3, 2, 0, 1)                                                                                                                                                                                                                                                                                                                                                                                                                                                                                                                                                |

continued on next page –

Table 9 – continued from previous page

|              |                                                                                |
|--------------|--------------------------------------------------------------------------------|
| $M_{2,6}^6$  | $m$ -vector: (88, 7, 1)                                                        |
| Perms.:      | (2, 4, 1, 5, 0, 3), (0, 5, 4, 3, 2, 1); (3, 5, 4, 0, 1, 2), (5, 4, 3, 2, 0, 1) |
| $M_{2,7}^6$  | $m$ -vector: (79, 8, 1)                                                        |
| Perms.:      | (5, 4, 1, 3, 0, 2), (0, 4, 3, 5, 2, 1); (1, 4, 5, 0, 3, 2), (2, 5, 1, 0, 4, 3) |
| $M_{2,8}^6$  | $m$ -vector: (79, 8, 1)                                                        |
| Perms.:      | (5, 4, 1, 3, 0, 2), (0, 4, 3, 5, 1, 2); (1, 4, 5, 0, 2, 3), (2, 5, 1, 0, 4, 3) |
| $M_{2,9}^6$  | $m$ -vector: (79, 8, 1)                                                        |
| Perms.:      | (4, 5, 1, 3, 0, 2), (0, 4, 3, 5, 1, 2); (1, 4, 5, 0, 3, 2), (3, 5, 2, 0, 4, 1) |
| $M_{2,10}^6$ | $m$ -vector: (79, 8, 1)                                                        |
| Perms.:      | (4, 5, 1, 3, 0, 2), (0, 4, 3, 5, 1, 2); (1, 4, 5, 0, 3, 2), (3, 5, 1, 0, 4, 2) |
| $M_{2,11}^6$ | $m$ -vector: (87, 9, 1)                                                        |
| Perms.:      | (5, 4, 3, 1, 0, 2), (2, 5, 4, 3, 0, 1); (5, 1, 0, 4, 3, 2), (3, 4, 5, 0, 2, 1) |
| $M_{2,12}^6$ | $m$ -vector: (87, 9, 1)                                                        |
| Perms.:      | (5, 4, 3, 1, 0, 2), (2, 5, 4, 3, 0, 1); (1, 5, 0, 4, 3, 2), (3, 4, 5, 0, 2, 1) |
| $M_{2,13}^6$ | $m$ -vector: (85, 42, 1)                                                       |
| Perms.:      | (1, 2, 0, 3, 4, 5), (0, 3, 1, 4, 2, 5); (1, 3, 2, 4, 0, 5), (2, 1, 0, 5, 4, 3) |

## References

- [1] B. A. Burton, B. Datta, N. Singh, J. Spreer, *A construction principle for tight and minimal triangulations of manifolds*. Preprint, 21 pages, 2 figures, arXiv:1511.04500 [math.GT], 2016.
- [2] F. Effenberger, J. Spreer, **simpcomp** – a GAP toolbox for simplicial complexes, *ACM Communications in Computer Algebra* **44 (4)** (2010), 186–189.
- [3] F. Effenberger, J. Spreer, **simpcomp** – a GAP toolkit for simplicial complexes, Version 2.1.6, 2009 – 2016, <https://github.com/simpcomp-team/simpcomp>.
